# Supplementary material for: Trainable, self-verifying variational quantum eigensolver using adiabatic warm starts
Source: arXiv:2602.17612 source file (2026-10-29)
Supplement: Supplementary file 1 [file supplemental.tex]

% ===========================
% Supplemental material
% ===========================
\documentclass[aps,pra,reprint,onecolumn,superscriptaddress]{revtex4-2}

% --- Packages ---
\usepackage{amsmath,amssymb,amsfonts}
\usepackage{bm}
\usepackage{mathtools}
\usepackage{physics}
\usepackage{graphicx}
\usepackage{xcolor}
\usepackage{microtype}
\usepackage{algorithm}
\usepackage{algpseudocode}
\usepackage{hyperref}
\hypersetup{colorlinks=true,linkcolor=blue,citecolor=blue,urlcolor=blue}

\usepackage{overpic}
\usepackage{orcidlink}

\usepackage{amsthm}
\usepackage{braket}
\theoremstyle{plain}

% --- Theorem environments ---
\newtheorem{theorem}{Theorem}
\newtheorem{assumption}{Assumption}
\newtheorem{lemma}{Lemma}
\newtheorem{corollary}{Corollary}
\newtheorem{remark}{Remark}

% --- Macros ---

\newcommand{\dl}{\delta\lambda}
\newcommand{\deltamin}{\Delta_{\rm min}}
\newcommand{\deltaminj}{\Delta^{j_\star}_{\rm min}}
\newcommand{\bth}{{\bm{\theta}}}
\newcommand{\nupdate}{N_{\rm updates}}
\newcommand{\bigo}{\mathcal{O}}
\newcommand{\aref}[1]{Assumption~\ref{#1}}
\newcommand{\tref}[1]{Theorem~\ref{#1}}
\newcommand{\lref}[1]{Lemma~\ref{#1}}
\newcommand{\eref}[1]{Eq.~\ref{#1}}
\newcommand{\sref}[1]{Section~\ref{#1}}
\newcommand{\cref}[1]{Corollary~\ref{#1}}
\newcommand{\bg}{\bm{g}}
\newcommand{\bG}{\mathbf{G}}
\newcommand{\bK}{\mathbf{K}}
\newcommand{\mH}{\mathcal{H}}

\newcommand{\Var}{\mathrm{Var}}
\newcommand{\Std}{\sigma}
\newcommand{\nh}{\mathcal{K}}

% Usual (decimal) numbering
\renewcommand{\thesection}{\arabic{section}}
\renewcommand{\thesubsection}{\thesection.\arabic{subsection}}

% Fix references
\makeatletter
\renewcommand{\p@subsection}{}
\renewcommand{\p@subsubsection}{}
\makeatother

% hide subsections (and deeper) from the ToC
\makeatletter
\def\l@subsection#1#2{}
\def\l@subsubsection#1#2{}
\def\l@paragraph#1#2{}      % optional
\def\l@subparagraph#1#2{}   % optional
\makeatother

% --- ORCID ---
\newcommand{\orcBojan}{\orcidlink{0000-0002-5085-2506}}
\newcommand{\orcMarco}{\orcidlink{0000-0002-3215-3453}}
\newcommand{\orcLewis}{\orcidlink{0009-0006-1595-102X}}
\newcommand{\orcMichael}{\orcidlink{0000-0002-2636-9936}}

% --- Affiliations ---
\newcommand{\affA}{\affiliation{University of Ljubljana, Faculty of Computer and Information Science, Ve\v{c}na pot 113, 1000 Ljubljana, Slovenia}}
\newcommand{\affB}{\affiliation{Rudolfovo, Science and Technology Centre, Novo mesto, Slovenia}}
\newcommand{\affC}{\affiliation{Quantinuum, Partnership House, Carlisle Place, London SW1P 1BX, United Kingdom}}

\begin{document}

% Title
\title{Supplemental Material:\\
Scalable, self-verifying variational quantum eigensolver using adiabatic warm starts}

% --- Authors ---
\author{Bojan Žunkovič\orcBojan}\email{bojan.zunkovic@fri.uni-lj.si}\affA\affB
\author{Marco Ballarin\orcMarco}\affC
\author{Lewis Wright\orcLewis}\affC
\author{Michael Lubasch\orcMichael}\email{michael.lubasch@quantinuum.com}\affC

\date{February 19, 2026}

\setcounter{section}{0}
\renewcommand{\thesection}{S\arabic{section}}
\renewcommand{\thesubsection}{S\arabic{section}.\arabic{subsection}}
\renewcommand{\theequation}{S\arabic{section}.\arabic{equation}}

\maketitle

In this supplemental material, we first define the setup and notation.
Then we prove both theorems of the main text as well as the absence of barren plateaus.
Then we show how to extend our results assuming $\epsilon$-exact representability.
Finally, we carry out a detailed shot-noise analysis.

\setcounter{tocdepth}{1}
\tableofcontents

% ======================================================
\section{Setup and notation}\label{sec: setup}
% ======================================================
We consider the Hamiltonian
\begin{equation}
H(\lambda) = (1-\lambda)H_\text{i} + \lambda H_\text{f},
\qquad \lambda\in[0,1],
\end{equation}
that interpolates between the initial Hamiltonian $H_\text{i}$ and the target final Hamiltonian $H_\text{f}$.
We define the instantaneous ground state $\ket{\psi_0(\lambda)}$, spectral gap
\begin{equation}
\Delta(\lambda)=E_1(\lambda)-E_0(\lambda)
\end{equation}
where $E_0(\lambda)$ ($E_{1}(\lambda)$) denotes the instantaneous ground (first-excited-state) energy, and minimum spectral gap
\begin{equation}
\deltamin = \min_{\lambda\in[0,1]}\Delta(\lambda).
\end{equation}

A variational family $\{\ket{\psi(\bth)}\}$ is assumed to exactly represent $\ket{\psi_0(\lambda)}$ for all $\lambda$.

The variational energy is
\begin{equation}
E_\lambda(\bth)
=
\bra{\psi(\bth)} H(\lambda) \ket{\psi(\bth)},
\end{equation}
with minimizer $\bth^\star(\lambda)$.
We assume smooth dependence on $\lambda$ and bounded operator norms for $H(\lambda)$ and its derivatives.

The local behaviour of the variational landscape can be characterized with the help of the geometric tensor
\begin{equation}
g_{\mu\nu}(\bth(\lambda)) = \mathrm{Re}\!\left( \langle \partial_\mu \psi | \partial_\nu \psi \rangle - \langle \partial_\mu \psi | \psi \rangle \langle \psi | \partial_\nu \psi \rangle \right).
\end{equation}

We aim to optimize the variational energy in steps. Therefore, we discretize the adiabatic path into $T$ slices,
\begin{equation}
\lambda_t = t \, \delta \lambda, \qquad \delta \lambda = \frac{1}{T}, \qquad t=0,1,\dots,T,
\end{equation}
and carry out the optimization iteratively along the path by making use of warm starts.
We choose $\bth_{0}$ to satisfy $\ket{\psi(\bth^\star)}=\ket{\psi_0(0)}$.
Then, for each slice $t=1,\dots,T$, we apply a gradient-based optimizer $K$ times to minimize $E_{\lambda_{t}}$ using the variational circuit initialized with the previously optimized parameters $\bth_{t-1}$:
\begin{align}
\bth_{t}^{(0)} &= \bth_{t-1}^{(K)}, \\ \nonumber
\bth_{t}^{(k+1)} &= \bth_{t}^{(k)} - \eta\, \bm{\mathcal{G}}_{t}\!\left(\bth_{t}^{(k)}\right), \qquad k=0,1,\dots,K-1, \\
\ket{\psi_t} &= \ket{\psi(\bth_t^{(K)})},
\end{align}
where $\eta>0$ is the learning rate and $-\bm{\mathcal{G}}_{t}(\bth)$ the chosen descent direction at $\lambda=\lambda_{t}$.
For the descent direction, we can use vanilla gradient descent, i.e.\ $\bm{\mathcal{G}}_{t}(\bth)=\nabla_\bth E_{\lambda_{t}}(\bth)$, or more advanced gradient-based optimizers.
In total, our approach performs $\nupdate=TK$ optimization steps.

To obtain our guarantees for \texttt{Theorem~1} of the main paper, we use the assumptions:
\begin{assumption}[Spectral gap]
The instantaneous ground state of $H(\lambda)$ is nondegenerate and $\deltamin>0$.
\end{assumption}
\begin{assumption}[Exact representability]
\label{supp: ass: exact rep}
For all $\lambda\in[0,1]$, there exists $\bth^\star(\lambda)$ such that
\begin{equation}
\ket{\psi(\bth^\star(\lambda))}=\ket{\psi_0(\lambda)}.
\end{equation}
\end{assumption}
\begin{assumption}[Nondegenerate geometry]\label{supp: ass: geometry}
There exists a constant $\gamma>0$ such that, for all $\lambda\in[0,1]$ and all $\bth^\star(\lambda)$, the geometric tensor satisfies
\begin{equation}
\bg(\bth^\star(\lambda))\succeq \gamma\,\mathbb{I}.
\end{equation}
\end{assumption}

% ======================================================
\subsection{Variational ansatz and derivatives}\label{sec: derivatives}
% ======================================================
In the main text and throughout this supplemental material, we utilize a variational ansatz with $M$ parameters over $n$ qubits:
\begin{align}
    \ket{\psi(\bth)}=U_{M-1}U_{M-2}\dots U_1U_0\ket{0}, \quad U_j=e^{-iP_j\theta_j}, \quad P_j\in\{I,X,Y,Z\}^{\otimes n}.
\end{align}
We can express the first derivative of this ansatz as:
\begin{align}
    \frac{\partial \ket{\psi(\bth)}}{\partial \theta_k}&=U_{M-1}\dots U_{k+1} (-iP_k) U_k\dots U_0\ket{0} \\
    &=-i U_{M-1}\dots U_{k+1}\;P_k\;(U_{M-1}\dots U_{k+1})^{\dagger} U_{M-1}\dots U_{k+1}U_k\dots U_0\ket{0}\\
    &=-i \widetilde{P_k}\ket{\psi(\bth)}.
\end{align}
We thus have a Pauli operator $\widetilde{P}_k$ that is evolved in the Heisenberg picture by all the unitaries that follow it. It is also important to note that $\widetilde{P}_k$ is Hermitian:
\begin{align}
    \widetilde{P}_k=U_{M-1}\dots U_{k+1}\;P_k\;(U_{M-1}\dots U_{k+1})^{\dagger} =\widetilde{P}_k^{\dagger}.
\end{align}
For the second derivative, for $l > k$, we get:
\begin{align}
    \frac{\partial^2 \ket{\psi(\bth)}}{\partial \theta_k\partial\theta_l}&=U_{M-1}\dots U_{l+1} (-iP_l) U_l\dots U_{k+1} (-iP_k) U_k\dots U_0\ket{0}\\
    &=-U_{M-1}\dots U_{l+1} P_l (U_{M-1}\dots U_{l+1})^{\dagger} U_{M-1}\dots U_{l+1}U_l\dots U_{k+1} P_k (U_{M-1}\dots U_{k+1})^{\dagger} U_{M-1}\dots U_{k+1}U_k\dots U_0\ket{0}\\
    &=-\widetilde{P}_l\widetilde{P}_k\ket{\psi(\bth)}.
\end{align}
Note that if $l=k$, the double derivative simplifies to:
\begin{align}
    \frac{\partial^2 \ket{\psi(\bth)}}{\partial \theta_k\partial\theta_k}&=-\ket{\psi(\bth)}.
\end{align}
We compute the energy gradients:
\begin{align}
    \frac{\partial \expval{H}}{\partial \theta_k}&=\frac{\partial\bra{\psi(\bth)}H\ket{\psi(\bth)}}{\partial\theta_k}=\frac{\partial\bra{\psi(\bth)}}{\partial\theta_k}H\ket{\psi(\bth)}+\partial\bra{\psi(\bth)}H\frac{\ket{\psi(\bth)}}{\partial\theta_k} \\
    &=i\bra{\psi(\bth)}\widetilde{P}_kH\ket{\psi(\bth)} - i\bra{\psi(\bth)}H\widetilde{P}_k\ket{\psi(\bth)} \\
    &= i\bra{\psi(\bth)}[\widetilde{P}_k,H]\ket{\psi(\bth)} \\
    &= 2\Im{\bra{\psi(\bth)}H\widetilde{P}_k\ket{\psi(\bth)} }.
\end{align}

\medskip

We compute the off-diagonal elements of the Hessian:
\begin{align}
    \frac{\partial^2 \expval{H}}{\partial \theta_k\partial\theta_l}&= \frac{\partial^2\bra{\psi(\bth)}}{\partial\theta_k\partial\theta_l}H\ket{\psi(\bth)}+\frac{\partial\bra{\psi(\bth)}}{\partial\theta_k}H\frac{\ket{\psi(\bth)}}{\partial\theta_l} +\frac{\partial\bra{\psi(\bth)}}{\partial\theta_l}H\frac{\ket{\psi(\bth)}}{\partial\theta_k} +\bra{\psi(\bth)}H\frac{\partial^2\ket{\psi(\bth)}}{\partial\theta_k\partial\theta_l} \\
    &=- \bra{\psi(\bth)} \widetilde{P}_k\widetilde{P}_lH\ket{\psi(\bth)}+\bra{\psi(\bth)}\widetilde{P}_kH\widetilde{P}_l\ket{\psi(\bth)}+\bra{\psi(\bth)}\widetilde{P}_lH\widetilde{P}_k\ket{\psi(\bth)}-\bra{\psi(\bth)}H\widetilde{P}_l\widetilde{P}_k\ket{\psi(\bth)} \\
    &= \bra{\psi(\bth)}\Big[\widetilde{P}_k,\big[H,\widetilde{P}_l\big]\Big]\ket{\psi(\bth)},
\end{align}
and the diagonal elements:
\begin{align}
    \frac{\partial^2 \expval{H}}{\partial \theta_k\partial\theta_k}&=-2\expval{H}+2 \bra{\psi(\bth)}\widetilde{P}_kH\widetilde{P}_k\ket{\psi(\bth)}.
\end{align}

Finally, the third derivatives of the energy with respect to the variational parameters read:
\begin{align}
    \frac{\partial^3 \expval{H}}{\partial \theta_m\partial\theta_l\partial\theta_k}&=-i\expval{
    \Big[
    \big[\widetilde{P}_m,\widetilde{P}_k\big],
    \big[\widetilde{P}_l,H\big]
    \Big] +
    \Big[
    \big[\widetilde{P}_k,\widetilde{P}_l\big],
    \big[\widetilde{P}_m,H\big]
    \Big] +
    \Big[
    \big[\widetilde{P}_l,\widetilde{P}_m\big],
    \big[\widetilde{P}_k,H\big]
    \Big] 
    }_{\bth}
\end{align}

% ======================================================
\section{Proof of Theorem 1: Geometric formulation of adiabatic tracking}\label{sec: pl proof}
% ======================================================
In this section, we establish \texttt{Theorem 1} of the main text by a sequence of lemmas, based on standard deep-learning techniques, exact smoothness, and Lipschitz bounds arising from the particular choice of the variational ansatz. The algorithm proceeds by first shifting the adiabatic parameter $\lambda$ by a small amount $\dl$, ensuring that the previously optimised state lies in a well-behaved region of the new landscape, which guarantees linear convergence to a unique optimum. 

\medskip
\noindent
\texttt{Proof roadmap:} 
\begin{enumerate}
\item \textbf{Derivative structure and smoothness.}
\lref{lem: derivatives} gives explicit formulas for the gradient and Hessian for the assumed variational ansatz. The subsequent Smoothness \lref{lem: smoothness} establishes global $L$--smoothness, and the Hessian Lipschitz \lref{lem: hessian lipschitz} proves that the Hessian varies in a controlled manner with Lipschitz constant $L_H$. These lemmas provide bounds on how fast the local optimization landscape properties can change.

\item \textbf{Curvature at the minimum.}
The Hessian lower bound \lref{lem: hess lower bound} shows that at $\bth^\star(\lambda)$ the Hessian is uniformly positive definite, with a lower bound determined by the spectral gap and the nondegeneracy constant of the variational metric. This provides a well-behaved optimization landscape at the variational minimum.

\item \textbf{Local PŁ inequality}
The Local Polyak--\L{}ojasiewicz \lref{lem: PŁ inequality} combines the curvature lower bound (\lref{lem: hess lower bound}) with Hessian Lipschitz continuity (\lref{lem: hessian lipschitz}) to identify a neighborhood in which the PŁ inequality holds.

\item \textbf{Adiabatic drift and linear contraction}
\lref{lem:drift-bound} bounds the drift of the minimizer, i.e., how much $\bth^\star(\lambda)$ changes under a change of $\lambda$. This can be used together with the \lref{lem: PŁ inequality} to show linear convergence of the energy error after a sufficiently small step $\dl$, summarised in the warm-start \lref{lem: warm-start}.

\item \textbf{Tracking error}
The local warm-start \lref{lem: warm-start} and the adiabatic drift bound \lref{lem:drift-bound} are then combined to derive \texttt{Theorem 1} from the main manuscript. We distinguish two boundary regimes:
\begin{itemize}
\item \texttt{Option 1:} larger step size $\dl$ and \textit{many} optimization steps for a fixed $\lambda$ -- discussed in \sref{sec:daws1}; 
\item \texttt{Option 2:} smaller step size $\dl$ and only \textit{one} optimization step for a fixed $\lambda$ -- discussed in \sref{sec:daws2}. 
\end{itemize}
In both cases, we obtain the same scaling of total complexity, with a slightly different resource allocation. In \texttt{option 1}, we show that $\dl\propto\deltamin^2$ and the number of gradient steps $K\propto1/\deltamin$, providing the $1/\deltamin^3$ scaling. In \texttt{option 2}, we take only one gradient update step (i.e., $K=1$) but have to use more slices, namely $\dl\propto\deltamin^3$. Both variants also yield the same total complexity with respect to other physical parameters, but differ slightly in their numerical constants. \texttt{Theorem 1} of the main text is for simplicity structured to be in line with the \texttt{option 1}, but it could equally well be written in terms of the \texttt{option 2}.
\end{enumerate}

% ======================================================
\subsection{Lemmas and linear convergence theorem}
% ======================================================

\begin{lemma}[Derivatives]
\label{lem: derivatives}
The gradient and Hessian satisfy
\begin{align}
\partial_{\theta_k}E(\bth)
&= i\langle\psi|[\widetilde P_k,H]|\psi\rangle,\\
\partial_{\theta_k}\partial_{\theta_l}E(\bth)
&=\langle\psi|[\widetilde P_k,[H,\widetilde P_l]]|\psi\rangle,
\end{align}
where $\widetilde P_k$ denotes the conjugate generator.
\end{lemma}
\begin{proof}
These expressions were proven in \sref{sec: derivatives}.
\end{proof}

\begin{lemma}[Smoothness]
\label{lem: smoothness}
The energy $E_\lambda(\bth)$ is $L$-smooth with
\begin{align}
L = \sup_{\bth} \| \nabla^2 E(\bth) \|_{\mathrm{op}} \le 4 \|H\|_{\mathrm{op}} M .
\end{align}
\end{lemma}

\begin{proof}
From \lref{lem: derivatives}, the Hessian entries are given by
\begin{align}
\partial_{\theta_k}\partial_{\theta_l} E(\bth) = \langle \psi(\bth) | [\widetilde P_k,[H,\widetilde P_l]] | \psi(\bth) \rangle ,
\end{align}
where $\widetilde P_k = U_{>k} P_k U_{>k}^{\rm opt}$ denotes the conjugated generator. ach $\widetilde P_k$ is Hermitian and unitary, hence $\|\widetilde P_k\|_{\mathrm{op}}=1$. To bound the operator norm of the Hessian, we use the variational characterization
\begin{align}
\| \nabla^2 E(\bth) \|_{\mathrm{op}} = \sup_{\|v\|_2 = 1}| v^\top \nabla^2 E(\bth)\, v |.
\end{align}
For any $v \in \mathbb{R}^M$ with $\|v\|_2 = 1$, define the operator
\begin{align}
A(v) = \sum_{k=1}^{M} v_k \widetilde P_k .
\end{align}
Using the bilinearity of the Hessian, we obtain
\begin{align}
v^\top \nabla^2 E(\bth)\, v
&= \sum_{k,l} v_k v_l \langle \psi | [\widetilde P_k,[H,\widetilde P_l]] | \psi \rangle \\
&= \langle \psi | [A(v),[H,A(v)]] | \psi \rangle .
\end{align}
Taking the absolute value and using that expectation values are bounded by the operator norm yields
\begin{align}
\left| \langle \psi | [A(v),[H,A(v)]] | \psi \rangle \right| \le \| [A(v),[H,A(v)]] \|_{\mathrm{op}} .
\end{align}
We now bound the double commutator using the general inequality
$\|[X,Y]\|_{\mathrm{op}} \le 2\|X\|_{\mathrm{op}}\|Y\|_{\mathrm{op}}$:
\begin{align}
\| [A,[H,A]] \|_{\mathrm{op}}
&\le 2 \|A\|_{\mathrm{op}} \|[H,A]\|_{\mathrm{op}} \\
&\le 2 \|A\|_{\mathrm{op}} \cdot 2 \|H\|_{\mathrm{op}} \|A\|_{\mathrm{op}} = 4 \|H\|_{\mathrm{op}} \|A\|_{\mathrm{op}}^2 .
\end{align}
It remains to bound $\|A(v)\|_{\mathrm{op}}$. Since each $\widetilde P_k$ is unitary,
\begin{align}
\|A(v)\|_{\mathrm{op}} &\le \sum_{k=1}^{M} |v_k| \|\widetilde P_k\|_{\mathrm{op}} \\
&= \sum_{k=1}^{M} |v_k| \le \|v\|_1 \le \sqrt{M}\, \|v\|_2 .
\end{align}
For $\|v\|_2=1$, this implies
\begin{align}
\|A(v)\|_{\mathrm{op}}^2 \le M .
\end{align}
Combining the above bounds, we conclude that for all unit vectors $v$,
\begin{align}
|v^\top \nabla^2 E(\bth)\, v| \le 4 \|H\|_{\mathrm{op}} M .
\end{align}
Taking the supremum over $v$ yields
\begin{align}
\|\nabla^2 E(\bth)\|_{\mathrm{op}} \le 4 \|H\|_{\mathrm{op}} M ,
\end{align}
uniformly in $\bth$.
\end{proof}

\begin{lemma}[Hessian Lipschitz continuity]
\label{lem: hessian lipschitz}
For all $\bth,\bth' \in \mathbb{R}^M$, the Hessian of the variational energy satisfies
\begin{align}
\|\nabla^2 E(\bth') - \nabla^2 E(\bth)\|_{\mathrm{op}} \le L_H \|\bth' - \bth\|_2 ,
\end{align}
with Lipschitz constant
\begin{align}
L_H = 24\|H\|_{\mathrm{op}} M^{3/2}.
\end{align}
\end{lemma}

\begin{proof}
We interpolate linearly between the two parameter points by defining
\begin{align}
\bth(t) = \bth + t(\bth' - \bth),
\end{align}
with $t \in [0,1]$.
By the fundamental theorem of calculus,
\begin{align}
\nabla^2 E(\bth') - \nabla^2 E(\bth) = \int_0^1 \frac{d}{dt} \nabla^2 E(\bth(t))\,dt .
\end{align}
Taking the operator norm and applying the triangle inequality yields
\begin{align}
\|\nabla^2 E(\bth') - \nabla^2 E(\bth)\|_{\mathrm{op}} \le \int_0^1 \left\| \frac{d}{dt} \nabla^2 E(\bth(t)) \right\|_{\mathrm{op}} dt .
\end{align}
The derivative of the Hessian along the path can be written using the chain rule as
\begin{align}
\frac{d}{dt} \nabla^2 E(\bth(t)) = \sum_{m=1}^M (\bth'_m - \bth_m)\, \nabla^3_m E(\bth(t)) .
\end{align}
Taking norms gives
\begin{align}
\left\| \frac{d}{dt} \nabla^2 E(\bth(t)) \right\|_{\mathrm{op}} \le \sum_{m=1}^M |\bth'_m - \bth_m|\, \|\nabla^3_m E(\bth(t))\|_{\mathrm{op}} .
\end{align}
Applying Cauchy--Schwarz to the sum over $m$ produces the first $\sqrt{M}$ factor:
\begin{align}
\sum_{m=1}^M |\bth'_m - \bth_m| \le \sqrt{M}\,\|\bth' - \bth\|_2 .
\end{align}
Hence,
\begin{align}
\left\| \frac{d}{dt} \nabla^2 E(\bth(t)) \right\|_{\mathrm{op}} \le \sqrt{M}\,\|\bth' - \bth\|_2 \max_m \|\nabla^3_m E(\bth(t))\|_{\mathrm{op}} .
\end{align}
We now bound $\|\nabla^3_m E(\bth)\|_{\mathrm{op}}$.
From the explicit third-derivative formula, each component has the structure
\begin{align}
\partial_{\theta_m}\partial_{\theta_k}\partial_{\theta_l} E(\bth) = \langle \psi | [[\widetilde P_m,\widetilde P_k],[\widetilde P_l,H]] | \psi \rangle + \text{permutations}.
\end{align}
The operator norm of $\nabla^3_m E$ is obtained by taking the supremum over unit vectors $u,v \in \mathbb{R}^M$:
\begin{align}
\|\nabla^3_m E(\bth)\|_{\mathrm{op}} = \sup_{\|u\|_2=\|v\|_2=1} \left| \sum_{k,l=1}^M u_k v_l \partial_{\theta_m}\partial_{\theta_k}\partial_{\theta_l} E(\bth) \right| .
\end{align}
Using Cauchy--Schwarz twice yields the second source of $M$:
\begin{align}
\sum_{k,l=1}^M |u_k||v_l| \le \|u\|_1 \|v\|_1 \le M .
\end{align}
Each nested commutator term satisfies
\begin{align}
\|[[\widetilde P_m,\widetilde P_k],[\widetilde P_l,H]]\|_{\mathrm{op}} \le 8 \|H\|_{\mathrm{op}},
\end{align}
since $\|\widetilde P_j\|_{\mathrm{op}}=1$ and $\|[X,Y]\|_{\mathrm{op}} \le 2\|X\|_{\mathrm{op}}\|Y\|_{\mathrm{op}}$.
Accounting for the three permutations appearing in the third derivative gives
\begin{align}
\|\nabla^3_m E(\bth)\|_{\mathrm{op}} \le 24 \|H\|_{\mathrm{op}} M .
\label{eq: nabla^3 bound}
\end{align}
Substituting this bound back, we obtain
\begin{align}
\left\| \frac{d}{dt} \nabla^2 E(\bth(t)) \right\|_{\mathrm{op}} \le 24 \|H\|_{\mathrm{op}} M^{3/2} \|\bth' - \bth\|_2 .
\end{align}
Finally, integrating over $t \in [0,1]$ yields
\begin{align}
\|\nabla^2 E(\bth') - \nabla^2 E(\bth)\|_{\mathrm{op}} \le 24 \|H\|_{\mathrm{op}} M^{3/2} \|\bth' - \bth\|_2 .
\end{align}
\end{proof}

\begin{lemma}[Hessian lower bound] 
\label{lem: hess lower bound}
At the variational minimum $\bth^\star(\lambda)$, the Hessian of the energy satisfies
\begin{equation}
    \nabla^2 E_\lambda(\bth^\star(\lambda)) \succeq 2\gamma\deltamin I.
\end{equation}
\end{lemma}

\begin{proof}
We evaluate the Hessian at the variational minimum $\bth^\star$ where $|\psi(\bth^\star)\rangle = |0\rangle$ is the nondegenerate ground state of $H(\lambda)$ with eigenvalue $E_0$. Let $v \in \mathbb{R}^M$ be an arbitrary unit vector with $\|v\|_2 = 1$.

Using the Hessian formula from Lemma 1, we write the quadratic form as
\begin{equation}
    v^\top \nabla^2 E(\bth^\star) v = \sum_{k,l=1}^M v_k v_l \langle 0 | [\widetilde{P}_k, [H, \widetilde{P}_l]] | 0 \rangle.
\end{equation}
Define the operator $A(v) = \sum_{k=1}^M v_k \widetilde{P}_k$. By bilinearity of the commutator, this yields
\begin{equation}
    v^\top \nabla^2 E(\bth^\star) v = \langle 0 | [A(v), [H, A(v)]] | 0 \rangle.
\end{equation}
Using the identity $[A, [H, A]] = 2A(H-E_0)A - \{A^2, (H-E_0)\}$ and the fact that $(H-E_0)|0\rangle = 0$, the second term vanishes in the expectation value, leaving
\begin{equation}
    \langle 0 | [A, [H, A]] | 0 \rangle = 2 \langle 0 | A (H-E_0) A | 0 \rangle.
\end{equation}
We insert a complete set of energy eigenstates $\{|n\rangle\}_{n \ge 0}$. Since the term for $n=0$ vanishes (as $E_0 - E_0 = 0$), the sum restricts to the excited subspace:
\begin{equation}
    2 \langle 0 | A (H-E_0) A | 0 \rangle = 2 \sum_{n \ge 1} (E_n - E_0) |\langle n | A | 0 \rangle|^2.
\end{equation}
Using the uniform spectral gap assumption $E_n - E_0 \ge \deltamin$ for all $n \ge 1$, we obtain:
\begin{align}
    v^\top \nabla^2 E(\bth^\star) v &\ge 2\deltamin \sum_{n \ge 1} |\langle n | A | 0 \rangle|^2 \\
    &= 2\deltamin \left( \sum_{n \ge 0} |\langle n | A | 0 \rangle|^2 - |\langle 0 | A | 0 \rangle|^2 \right) \\
    &= 2\deltamin \left( \langle 0 | A^2 | 0 \rangle - \langle 0 | A | 0 \rangle^2 \right).
\end{align}
The term in the parentheses is exactly the variance of the operator $A$ with respect to the ground state. This corresponds to the Fubini-Study metric, which projects the derivatives onto the tangent space orthogonal to $|0\rangle$:
\begin{equation}
    \text{Var}(A) = \sum_{k,l} v_k v_l \left( \langle 0 | \widetilde{P}_k \widetilde{P}_l | 0 \rangle - \langle 0 | \widetilde{P}_k | 0 \rangle \langle 0 | \widetilde{P}_l | 0 \rangle \right) = v^\top \bg(\bth^\star) v.
\end{equation}
By assumption, the ansatz is non-degenerate such that $\bg(\bth^\star) \succeq \gamma I$, which implies $v^\top \bg(\bth^\star) v \ge \gamma$. Therefore:
\begin{equation}
    v^\top \nabla^2 E(\bth^\star) v \ge 2\gamma\deltamin.
\end{equation}
Since this bound holds for all unit vectors $v$, we conclude
\begin{equation}
    \nabla^2 E(\bth^\star) \succeq 2\gamma\deltamin I.
\end{equation}
\end{proof}

\begin{lemma}[Local Polyak--Łojasiewicz inequality]
\label{lem: PŁ inequality}
Let $\bth^\star$ denote the variational minimum at fixed $\lambda$.
For
\begin{align}
\|\bth - \bth^\star\|_2 \le r_{\mathrm{PL}} = \frac{\gamma \deltamin}{L_H},
\end{align}
the Polyak--Łojasiewicz inequality holds:
\begin{align}
\frac{1}{2}\|\nabla E(\bth)\|_2^2 \ge \gamma \deltamin \big( E(\bth) - E(\bth^\star) \big).
\end{align}
\end{lemma}

\begin{proof}
We begin by recalling from Lemma~4 that the Hessian at the minimum satisfies
\begin{align}
\nabla^2 E(\bth^\star) \succeq 2 \gamma \deltamin I .
\end{align}
By Lemma~3, the Hessian is Lipschitz continuous with constant $L_H$, meaning
\begin{align}
\|\nabla^2 E(\bth) - \nabla^2 E(\bth^\star)\|_{\mathrm{op}} \le L_H \|\bth - \bth^\star\|_2 .
\end{align}
Since the Hessian is symmetric, we obtain a lower bound $\bth$:
\begin{align}
\nabla^2 E(\bth) \succeq \nabla^2 E(\bth^\star) - \|\nabla^2 E(\bth) - \nabla^2 E(\bth^\star)\|_{\mathrm{op}} I .
\end{align}
Substituting the previous bounds yields
\begin{align}
\nabla^2 E(\bth) \succeq \big( 2\gamma\deltamin - L_H \|\bth - \bth^\star\|_2 \big) I .
\end{align}
If $\|\bth - \bth^\star\|_2 \le \gamma\deltamin / L_H$, then
\begin{align}
2\gamma\deltamin - L_H \|\bth - \bth^\star\|_2 \ge \gamma\deltamin ,
\end{align}
and hence
\begin{align}
\nabla^2 E(\bth) \succeq \gamma \deltamin I .
\end{align}
Therefore, the energy is $\gamma\deltamin$--strongly convex in this neighborhood. Strong convexity implies the following quadratic lower bound on the function:
\begin{align}
E(\bth) - E(\bth^\star) \le \frac{1}{2\gamma\deltamin} \|\nabla E(\bth)\|_2^2 .
\end{align}
Rearranging this inequality yields
\begin{align}
\frac{1}{2}\|\nabla E(\bth)\|_2^2 \ge \gamma\deltamin \big( E(\bth) - E(\bth^\star) \big),
\end{align}
which is exactly the Polyak--Łojasiewicz inequality. Since all steps hold whenever $\|\bth - \bth^\star\|_2 \le r_{\mathrm{PL}}$, the claim follows.
\end{proof}

\begin{lemma}[Drift bound]
\label{lem:drift-bound}
Let $\bth^\star(\lambda)$ denote the variational minimizer of
\begin{align}
E_\lambda(\bth) = \langle \psi(\bth) | H(\lambda) | \psi(\bth) \rangle .
\end{align}
Assume that the Hessian at the minimum satisfies
\begin{align}
\nabla^2_\bth E_\lambda(\bth^\star(\lambda)) \succeq 2\gamma\deltamin I ,
\end{align}
and that $\|\widetilde P_k\|_{\mathrm{op}} = 1$ for all generators.
Then, for sufficiently small $\delta\lambda$,
\begin{align}
\|\bth^\star(\lambda+\delta\lambda) - \bth^\star(\lambda)\|_2 \le D\delta\lambda + O(\delta\lambda^2), \qquad D=\frac{\sqrt{M}\,\|\partial_\lambda H(\lambda)\|_{\mathrm{op}}}{\gamma\deltamin}.
\end{align}
\end{lemma}

\begin{proof}
At the variational minimum, the gradient vanishes:
\begin{align}
\nabla_\bth E_\lambda(\bth^\star(\lambda)) = 0 .
\end{align}
Differentiating with respect to $\lambda$ gives
\begin{align}
\frac{d}{d\lambda}\nabla_\bth E_\lambda(\bth^\star(\lambda)) = 0 .
\end{align}
Applying the chain rule yields
\begin{align}
\nabla^2_\bth E_\lambda(\bth^\star(\lambda))\,\dot{\bth}^\star(\lambda) + \nabla_\bth \partial_\lambda E_\lambda(\bth^\star(\lambda)) = 0 ,
\end{align}
where
\begin{align}
\dot{\bth}^\star(\lambda) = \frac{d}{d\lambda}\bth^\star(\lambda) .
\end{align}
Rearranging,
\begin{align}
\dot{\bth}^\star(\lambda) = -\big(\nabla^2_\bth E_\lambda(\bth^\star(\lambda))\big)^{-1}\nabla_\bth \partial_\lambda E_\lambda(\bth^\star(\lambda)) .
\end{align}
We first bound the inverse Hessian. From the assumed curvature lower bound,
\begin{align}
\nabla^2_\bth E_\lambda(\bth^\star(\lambda)) \succeq 2\gamma\deltamin I ,
\end{align}
it follows that
\begin{align}
\big\|\big(\nabla^2_\bth E_\lambda(\bth^\star(\lambda))\big)^{-1}\big\|_{\mathrm{op}} \le \frac{1}{2\gamma\deltamin} .
\end{align}
Next, we bound the gradient $\nabla_\bth \partial_\lambda E_\lambda$.
By definition,
\begin{align}
\partial_\lambda E_\lambda(\bth) = \langle \psi(\bth) | \partial_\lambda H(\lambda) | \psi(\bth) \rangle .
\end{align}
Differentiating with respect to $\theta_k$ yields
\begin{align}
\partial_{\theta_k}\partial_\lambda E_\lambda(\bth)
=
i\langle \psi(\bth)|[\widetilde P_k,\partial_\lambda H(\lambda)]|\psi(\bth)\rangle .
\end{align}
Using the commutator norm bound gives
\begin{align}
|\partial_{\theta_k}\partial_\lambda E_\lambda(\bth)| \le 2\|\partial_\lambda H(\lambda)\|_{\mathrm{op}} .
\end{align}
Therefore, the Euclidean norm of the gradient satisfies
\begin{align}
\|\nabla_\bth \partial_\lambda E_\lambda(\bth^\star(\lambda))\|_2 = \left(\sum_{k=1}^M |\partial_{\theta_k}\partial_\lambda E_\lambda|^2\right)^{1/2} \le 2\sqrt{M}\,\|\partial_\lambda H(\lambda)\|_{\mathrm{op}} .
\end{align}
Combining the bounds yields
\begin{align}
\|\dot{\bth}^\star(\lambda)\|_2 \le \frac{1}{2\gamma\deltamin}\,\|\nabla_\bth \partial_\lambda E_\lambda(\bth^\star(\lambda))\|_2 \le \frac{\sqrt{M}\,\|\partial_\lambda H(\lambda)\|_{\mathrm{op}}}{\gamma\deltamin} .
\end{align}
Finally, integrating over $\lambda \in [\lambda,\lambda+\delta\lambda]$ gives (since the assumed adiabatic schedule is linear in $\lambda$)
\begin{align}
\|\bth^\star(\lambda+\delta\lambda) - \bth^\star(\lambda)\|_2 \le \frac{\sqrt{M}\,\|\partial_\lambda H(\lambda)\|_{\mathrm{op}}}{\gamma\deltamin}\,\delta\lambda,
\end{align}
which proves the claim.
\end{proof}

\begin{lemma}[Adiabatic warm-start convergence]
\label{lem: warm-start}
Let 
\begin{align}
H(\lambda) &= (1-\lambda)H_\text{i} + \lambda H_\text{f} , \qquad \lambda\in[0,1],
\end{align}
and let 
\begin{align}
E_\lambda(\bth) &= \langle \psi(\bth)|H(\lambda)|\psi(\bth)\rangle
\end{align}
with a parametrized ansatz $|\psi(\bth)\rangle$ that exactly represents the ground state:
\begin{align}
|\psi(\bth^\star(\lambda))\rangle &= |\psi_0(\lambda)\rangle .
\end{align}
Assume only:
\begin{align}
E_1(\lambda)-E_0(\lambda) &\ge \deltamin > 0 \quad \forall\lambda , \\
\bg(\bth^\star(\lambda)) &\succeq \gamma I .
\end{align}
Then there exists an explicit constant $c>0$ such that, if
\begin{align}
\delta\lambda \le c\,\frac{\gamma^{2}\deltamin^2}{L_H \sqrt{M}\,\|\partial_\lambda H(\lambda)\|_{\mathrm{op}}},
\end{align}
the minimizer $\bth^\star(\lambda)$ lies in a Polyak--\L{}ojasiewicz (PŁ) region of $E_{\lambda+\delta\lambda}$.  

Within this region, gradient descent with step size $\eta \le 1/L$ converges linearly both in energy and in parameters:
\begin{align}
E_{\lambda+\delta\lambda}(\bth^{(k)}) - E_{\lambda+\delta\lambda}(\bth^\star)
&\le \left(1-\frac{\gamma\deltamin}{L}\right)^k \delta E_0 , \\
\|\bth^{(k)}-\bth^\star(\lambda+\delta\lambda)\|_2
&\le \left(1-\frac{\gamma\deltamin}{L}\right)^{k/2}
\|\bth^{(0)}-\bth^\star(\lambda+\delta\lambda)\|_2 .
\end{align}
In particular, to reach energy accuracy $\epsilon$, it suffices that the total number of optimization steps $K$ is
\begin{align}
K \ge \frac{L}{\gamma \deltamin} 
\ln \left( \frac{\delta E_0}{\epsilon} \right),
\end{align}
and the corresponding parameter error satisfies
\begin{align}
\|\bth^{(K)}-\bth^\star(\lambda+\delta\lambda)\|_2
\le \sqrt{\frac{2\epsilon}{\gamma\deltamin}} .
\end{align}
\end{lemma}

\begin{proof}
At $\bth^\star(\lambda)$ the gradient vanishes:
\begin{align}
\nabla_\bth E_\lambda(\bth^\star(\lambda)) = 0 .
\end{align}
From Lemma~\ref{lem:drift-bound},
\begin{align}
\|\bth^\star(\lambda+\delta\lambda)-\bth^\star(\lambda)\|_2 
\le \frac{\sqrt{M}\,\|\partial_\lambda H(\lambda)\|_{\mathrm{op}}}
{\gamma\deltamin}\,\delta\lambda .
\end{align}
Requiring this drift to be bounded by the PŁ radius 
$r_{\mathrm{PL}}=\gamma\deltamin/L_H$
yields the stated condition on $\delta\lambda$.

Inside the PŁ region, the energy is $\gamma\deltamin$--strongly convex and $L$--smooth. For one gradient descent step with $\eta=1/L$ we have by the gradient descent lemma~\cite{Ne18},
\begin{align}
E(\bth^{(k+1)}) 
\le E(\bth^{(k)}) - \frac{1}{2L}\|\nabla E(\bth^{(k)})\|_2^2 .
\end{align}
Applying the PŁ inequality
\begin{align}
\frac12 \|\nabla E(\bth)\|_2^2 
\ge \gamma\deltamin\big(E(\bth)-E(\bth^\star)\big),
\end{align}
and defining $\delta E_k=E(\bth^{(k)})-E(\bth^\star)$ gives
\begin{align}
\delta E_{k+1}
\le \left(1-\frac{\gamma\deltamin}{L}\right)\delta E_k .
\end{align}
Iterating yields
\begin{align}
\delta E_k 
\le \left(1-\frac{\gamma\deltamin}{L}\right)^k \delta E_0
\le e^{-k\frac{\gamma\deltamin}{L}}\delta E_0 .
\end{align}

Strong convexity additionally implies
\begin{align}
\frac{\gamma\deltamin}{2}
\|\bth-\bth^\star\|_2^2
\le E(\bth)-E(\bth^\star) .
\end{align}
Combining with the energy decay gives
\begin{align}
\|\bth^{(k)}-\bth^\star\|_2^2
\le \frac{2}{\gamma\deltamin}\delta E_k
\le \frac{2}{\gamma\deltamin}
\left(1-\frac{\gamma\deltamin}{L}\right)^k \delta E_0 ,
\end{align}
which yields linear convergence in parameters and the stated bound.
\end{proof}

% ======================================================
\subsection{Ground state tracking --- option 1}\label{sec:daws1}
% ======================================================

\subsubsection*{Discretization condition}
We discretize $\lambda$ so that consecutive minimizers lie within half of the PŁ radius:
\begin{align}
\|\bth^\star(\lambda_{k+1})-\bth^\star(\lambda_k)\|_2 \le \frac{r_{\mathrm{PL}}}{2}.
\end{align}
This is ensured provided
\begin{align}
\delta\lambda \le \frac{\gamma\deltamin}{2\sqrt{M}\|\partial_\lambda H\|_{\mathrm{op}}}\, r_{\mathrm{PL}} = \frac{\gamma^2\deltamin^2}{2L_H\sqrt{M}\|\partial_\lambda H\|_{\mathrm{op}}}.
\label{eq:delta-lambda-bound}
\end{align}

\subsubsection*{Warm--start entry into the PŁ region}
Assume that at step $t$ the iterate satisfies
\begin{align}
\|\bth_t-\bth^\star(\lambda_t)\|_2 \le \frac{r_{\mathrm{PL}}}{2}.
\end{align}
Then, using the triangle inequality,
\begin{align}
\|\bth_t-\bth^\star(\lambda_{t+1})\|_2
&\le \|\bth_t-\bth^\star(\lambda_t)\|_2 + \|\bth^\star(\lambda_t)-\bth^\star(\lambda_{t+1})\|_2 \\
&\le \frac{r_{\mathrm{PL}}}{2} + \frac{r_{\mathrm{PL}}}{2} = r_{\mathrm{PL}}.
\end{align}
Hence, the warm start always lies inside the PŁ region of the next energy landscape.

\subsubsection*{Gradient descent contraction}
Inside the PŁ region, by the \lref{lem: warm-start} the gradient descent with step size $\eta = 1/L$ satisfies
\begin{align}
\|\bth^{(k+1)}-\bth^\star\|_2 \le \sqrt{1-\frac{\gamma\deltamin}{L}} \|\bth^{(k)}-\bth^\star\|_2.
\end{align}
To reduce the error by a factor of $2$, i.e.
\begin{align}
\|\bth^{(k)}-\bth^\star\|_2 \le \frac{r_{\mathrm{PL}}}{2},
\end{align}
it suffices to choose $t$ such that
\begin{align}
\left(1-\frac{\gamma\deltamin}{L}\right)^{k/2} \le \frac12.
\end{align}
Using $\ln(1-x)\le -x$ for $x\in(0,1)$, we obtain
\begin{align}
k \ge K = \frac{2L}{\gamma\deltamin}\ln 2.
\label{eq:gd-steps}
\end{align}

\subsubsection*{Total complexity}
The total number of adiabatic steps is
\begin{align}
T = \frac{1}{\delta\lambda} = \frac{2L_H\sqrt{M}\|\partial_\lambda H\|_{\mathrm{op}}}{\gamma^2\deltamin^2}.
\end{align}
At each step, we perform $K$ gradient descent iterations as in \eqref{eq:gd-steps}. Therefore, the total number of gradient evaluations satisfies
\begin{align}
N_{\mathrm{grad}}
& =T \cdot K \\
& = \frac{4L_H\sqrt{M}\|\partial_\lambda H\|_{\mathrm{op}}}{\gamma^2\deltamin^2} \cdot \frac{L}{\gamma\deltamin}\ln 2.
\end{align}
Substituting $L\le 4\|H\|_{\mathrm{op}} M$, we finally obtain
\begin{align}
\nupdate
&\le \frac{16\ln 2}{\gamma^3} \, \frac{L_H\,\|H\|_{\mathrm{op}}\,M^{3/2}\,\|\partial_\lambda H\|_{\mathrm{op}}}{\deltamin^3}.
\end{align}
Inserting all constants, we find
\begin{align}
\boxed{\nupdate \le 384 \ln 2 \frac{M^3 \, \|H\|_{\mathrm{op}}^2 \, \|H_\text{f} - H_\text{i}\|_{\mathrm{op}}}{\gamma^3\deltamin^3}}
\end{align}

This is the protocol used in \texttt{Theorem 1} of the main manuscript. An alternative version is presented in the following subsection.

% ======================================================
\subsection{Ground state tracking --- option 2}\label{sec:daws2}
% ======================================================

In this section, we refine the warm-start analysis of \sref{sec:daws1} by explicitly tracking the \emph{transient optimization error} across adiabatic steps. Rather than requiring near-exact re-optimization at each step, we show that finite optimization effort per step suffices: the tracking error obeys a contractive recursion with an $\bigo(\dl)$ forcing term, yielding a uniform steady-state bound. In the end, we achieve the same level of optimization complexity with a slightly different analysis.

\subsubsection*{Forced contraction recursion}
We decompose the error after the $k$-th step:
\begin{align}
e_{t+1}
&= \bth^{(k=0)}-\bth^\star(\lambda_{t+1}) \\
&= \big(\bth^{(k=0)}-\bth^\star(\lambda_{t+1})\big) - \big(\bth^\star(\lambda_{t+1})-\bth^\star(\lambda_t)\big).
\end{align}
By \lref{lem: warm-start}, starting from $\bth^{(k=0)}$ and optimizing $E_{\lambda_{t+1}}$ for $K$ steps yields
\begin{align}
\|\bth^{(k=K)}-\bth^\star(\lambda_{t+1})\|_2 \le \rho^K \|\bth^{(k=0)}-\bth^\star(\lambda_{t+1})\|_2, \quad \rho=\sqrt{1-\frac{\gamma\deltamin}{2}}.
\end{align}
Using the triangle inequality and the drift bound,
\begin{align}
\|\bth_t^{(k=0)}-\bth^\star(\lambda_{t+1})\|_2
&\le \|\bth^{(k=0)}-\bth^\star(\lambda_t)\|_2 + \|\bth^\star(\lambda_{t+1})-\bth^\star(\lambda_t)\|_2 \\
&\le \|e_t\|_2 + D\,\delta\lambda + O(\delta\lambda^2).
\end{align}
Combining the last two inequalities, we find
\begin{align}
\|e_{t+1}\|_2 \le \rho^K \|e_t\|_2 + \rho^K D\,\delta\lambda + O(\delta\lambda^2).
\label{eq: forced contraction}
\end{align}

\subsubsection*{Uniform tracking error}
Iterating the recursion of \eref{eq: forced contraction} gives
\begin{align}
\|e_t\|_2
&\le (\rho^K)^t \|e_0\|_2  + \rho^K D\delta\lambda \sum_{j=0}^{t-1}(\rho^K)^j + O(\delta\lambda^2) \\
&\le (\rho^K)^t \|e_0\|_2 + \frac{\rho^K}{1-\rho^K} D\,\delta\lambda + O(\delta\lambda^2).
\end{align}
Since $1-\rho^K \approx K\gamma\deltamin/2L$ for small $\gamma\deltamin/L$ we find
\begin{align}
\|e_t\|_2 \le (\rho^K)^t \|e_0\|_2 + \frac{2L}{K\gamma\deltamin} D\,\delta\lambda + O(\delta\lambda^2).
\end{align}
In particular if $\|e_0\|_2=0$,
\begin{align}
\|e_t\|_2 \lesssim \frac{2L}{K}\,\frac{\sqrt{M}\,\|\partial_\lambda H(\lambda)\|_{\mathrm{op}}}{\gamma^2\deltamin^2}\,\delta\lambda .
\label{eq: uniform error bound}
\end{align}

\subsubsection*{Staying inside the PŁ region}
To ensure that the iterates never leave the PŁ region, it suffices that the steady-state error remains below $r_{\mathrm{PL}}/2$:
\begin{align}
\frac{2L}{t\,\gamma\deltamin}\,D\,\delta\lambda = \frac{2L}{K}\,\frac{\sqrt{M}\,\|\partial_\lambda H(\lambda)\|_{\mathrm{op}}}{\gamma^2\deltamin^2}\,\delta\lambda \le \frac{r_{\mathrm{PL}}}{2} = \frac{\gamma\deltamin}{2L_H}.
\end{align}
Equivalently, a sufficient discretization condition is
\begin{align}
\delta\lambda \le \frac{t\,\gamma^2\deltamin^2}{4L_H L}\,\frac{1}{D} = \bigo\!\left(\frac{t\,\gamma^3\deltamin^3}{L_H L\sqrt{M}\|\partial_\lambda H\|_{\mathrm{op}}} \right).
\end{align}
Under this condition, the warm-start iterations remain inside the PŁ region for all $k$, and the tracking error is uniformly bounded by \eref{eq: uniform error bound}.

\subsubsection*{Complexity}
Each adiabatic step requires $K$ gradient evaluations. The number of adiabatic steps is $T=1/\dl$. Hence, the total number of gradient evaluations satisfies
\begin{align}
\nupdate = KT = \frac{K}{\delta\lambda}
= \bigo\!\left(\frac{L_H L\sqrt{M}\|\partial_\lambda H\|_{\mathrm{op}}}{\gamma^3\deltamin^3} \right).
\end{align}
This yields the same asymptotic scaling as the analysis in \sref{sec:daws1}.

\subsubsection*{Explicit complexity for Pauli-generated ansätze}
Using the transient-error analysis framework, we evaluate the total gradient-update complexity $\nupdate$ by substituting the physical bounds derived in \sref{sec: derivatives} for a variational ansatz composed of $M$ Pauli-rotations. The total complexity is governed by the requirement that the steady-state tracking error remains within the Polyak--Łojasiewicz (PL) region, leading to the condition
\begin{equation}
\boxed{\nupdate \le 384\frac{M^3 \,\|H\|_{\mathrm{op}}^2 \, \|H_\text{f} - H_\text{i}\|_{\mathrm{op}}}{\gamma^3\deltamin^3}}.
\end{equation}

% ======================================================
\section{Proof of Theorem 1: Continuous-time adiabatic formulation and scaling}
% ======================================================
The proof of \texttt{Theorem 1} of the main text in the previous \sref{sec: pl proof} does not offer a clear picture of why we get an extra $1/\deltamin$ factor on the number of gradient steps $\nupdate$ in comparison to the expected $1/\deltamin^2$ adiabatic scaling of the time complexity.
In this section, we provide an alternative proof of the theorem using the time-dependent variational principle (TDVP). We demonstrate that, in the continuous-time formulation, the same scaling, $1/\deltamin^2$, is obtained. The extra $1/\deltamin$ factor comes from a \textit{stability requirement} of discrete numerical integration methods. This stability factor is required for both explicit and more stable implicit solvers. 

In the following, we first discuss the basics of the TDVP, then derive the continuous imaginary-time TDVP flow equations, and finally examine the numerical integration of the flow.

% ======================================================
\subsection{Variational manifold and geometric structures}
% ======================================================
We consider a smooth variational manifold
$\mathcal{M}\subset\mathbb{P}(\mathcal{H})$ embedded in projective Hilbert space,
parametrized by real coordinates
$\bth=(\theta_\mu)_{\mu=1}^{d}$, with associated normalized quantum states
$|\psi(\bth)\rangle \in \mathcal{H}$.
The geometry of $\mathcal{M}$ is inherited from the Fubini--Study metric. Define
tangent vectors~\cite{HaEtAl20}
\begin{align}
|\partial_\mu \psi\rangle = \frac{\partial}{\partial \theta_\mu} |\psi(\bth)\rangle, 
\qquad \langle \psi | \psi \rangle = 1.
\end{align}
The quantum geometric tensor
\begin{align}
Q_{\mu\nu} = \langle \partial_\mu \psi | \partial_\nu \psi \rangle - \langle \partial_\mu \psi | \psi \rangle \langle \psi | \partial_\nu \psi \rangle
\end{align}
induces a metric and a symplectic form:
\begin{align}
g_{\mu\nu} = \Re\, Q_{\mu\nu}, \qquad \omega_{\mu\nu} = 2\, \Im\, Q_{\mu\nu}.
\end{align}
On a Kähler manifold, these satisfy
\begin{align}
\omega_{\mu\nu} = - g_{\mu\sigma} J^\sigma{}_\nu
\end{align}
with $J^\sigma{}_\nu$ the complex structure. Denote by
\begin{align}
G^{\mu\nu}(\bth) = [\bg^{-1}]_{\mu\nu}(\bth)
\end{align}
the inverse metric.

% ======================================================
\subsection{Energy functional and TDVP flow}
% ======================================================
We again assume the setup defined in \sref{sec: setup}: the Hamiltonian depends smoothly on a dimensionless adiabatic parameter
$\lambda\in[0,1]$:
\begin{align}
H(\lambda) = (1-\lambda) H_\text{i} + \lambda H_\text{f}.
\end{align}
We again use the Assumptions 1-3 and define the energy functional on $\mathcal{M}$ by
\begin{align}
E(\bth,\lambda) = \langle \psi(\bth) | H(\lambda) | \psi(\bth) \rangle.
\end{align}
Physical time is $\tau \in [0,T]$, with linear schedule
\begin{align}
\lambda(\tau) = \frac{\tau}{T}.
\end{align}
The imaginary-time TDVP evolution is~\cite{HaEtAl20}
\begin{align}
\frac{d\theta_\mu}{d\tau} = - G^{\mu\nu}(\bth) \, \partial_\nu E(\bth,\lambda).
\label{eq:tdvp-flow}
\end{align}

% ======================================================
\subsection{Linearized TDVP dynamics}
% ======================================================
Let $\bth(\tau)$ be a solution of the TDVP equation \eqref{eq:tdvp-flow}, and let
\[
\delta\theta_\mu(\tau) = \theta_\mu(\tau) - \theta^\star_\mu(\lambda(\tau))
\]
denote the deviation from an instantaneous variational minimum $\bth^\star(\lambda)$.  
Differentiating $\delta\theta_\mu$ with respect to $\tau$ gives
\begin{align}
\frac{d}{d\tau} \delta\theta_\mu(\tau) 
= \frac{d\theta_\mu}{d\tau} - \frac{d}{d\tau} \theta^\star_\mu(\lambda(\tau))
= - G^{\mu\nu}(\bth) \,\partial_\nu E(\bth,\lambda) - \frac{1}{T} \, \partial_\lambda \theta^\star_\mu(\lambda),
\end{align}
where we used the TDVP flow \eqref{eq:tdvp-flow} and the linear schedule $\lambda(\tau) = \tau/T$.
By Taylor’s reminder theorem for multivariate functions, we have
\begin{align}
\partial_\nu E(\bth^\star + \delta\bth, \lambda)
= \partial_\nu E(\bth^\star, \lambda)
+ \mathcal{H}_{\sigma\nu}(\lambda) \, \delta\bth^\sigma
+ R_\nu(\delta\bth, \lambda),
\end{align}
where the Hessian at the minimum is
\[
\mathcal{H}_{\mu\nu}(\lambda) = \partial_\mu \partial_\nu E(\bth^\star(\lambda),\lambda),
\]
and the remainder $R_\nu$ satisfies the quadratic bound
\begin{align}
\|R(\delta\bth,\lambda)\|_2 \le \frac{1}{2} L_E \, \|\delta\bth\|_2^2,
\qquad
L_E = \sup_{\bth \in B(\bth^\star,r)} \|\nabla_\bth^3 E(\bth,\lambda)\|_\mathrm{op},
\end{align}
for $\|\delta\bth\|_2$ sufficiently small. Since $\bth^\star(\lambda)$ is a minimizer, $\partial_\nu E(\bth^\star,\lambda) = 0$, so
\begin{align}
\partial_\nu E(\bth,\lambda) = \mathcal{H}_{\sigma\nu}(\lambda) \, \delta\bth^\sigma + R_\nu(\delta\bth, \lambda).
\end{align}

Similarly, for the metric inverse $G^{\mu\nu}(\bth)$, we have
\begin{align}
G^{\mu\nu}(\bth) = G^{\mu\nu}(\bth^\star) + \Delta G^{\mu\nu}(\delta\bth), 
\qquad \|\Delta \bG(\delta\bth)\|_\mathrm{op} \le L_G \|\delta\bth\|_2,
\end{align}
with $L_G$ the Lipschitz constant of the metric. Substituting the expansions into the TDVP equation, we obtain
\begin{align}
\frac{d}{d\tau} \delta\theta_\mu
&= - \big(G^{\mu\nu}(\bth^\star) + \Delta G^{\mu\nu}(\delta\bth)\big) 
\big(\mathcal{H}_{\sigma\nu} \delta\bth^\sigma + R_\nu(\delta\bth,\lambda)\big) 
- \frac{1}{T} \partial_\lambda \theta^\star_\mu(\lambda) \\
&= K^\mu{}_\sigma(\lambda) \, \delta\bth^\sigma 
- \frac{1}{T} \partial_\lambda \theta^\star_\mu(\lambda) 
+ \underbrace{-\Delta G^{\mu\nu} \mathcal{H}_{\sigma\nu} \delta\bth^\sigma - (G^{\mu\nu} + \Delta G^{\mu\nu}) R_\nu}_{R^\mu(\delta\bth,\lambda)},
\end{align}
where we defined the linearized TDVP generator
\begin{align}
K^\mu{}_\sigma(\lambda) = - G^{\mu\nu}(\bth^\star(\lambda)) \, \mathcal{H}_{\nu\sigma}(\lambda),
\end{align}
and collected all higher-order nonlinear terms in
\begin{align}
R^\mu(\delta\bth,\lambda) = -\Delta G^{\mu\nu} \mathcal{H}_{\sigma\nu} \delta\bth^\sigma - (G^{\mu\nu} + \Delta G^{\mu\nu}) R_\nu(\delta\bth,\lambda).
\end{align}
By the submultiplicativity of the operator norm,
\begin{align}
\label{eq: tdvp bounds}
\|R(\delta\bth,\lambda)\|_2 \le C_\mathrm{nl} \, \|\delta\bth\|_2^2, 
\quad C_\mathrm{nl} = \frac{1}{2} L_E \|\bG\|_\mathrm{op} + L_G \|\mathcal{H}\|_\mathrm{op}.
\end{align}
The deviation from the instantaneous minimizer thus satisfies
\begin{align}\label{eq: tdvp reminder}
\boxed{
\frac{d}{d\tau} \delta\bth(\tau) = \bK(\lambda) \, \delta\bth(\tau) 
- \frac{1}{T} \partial_\lambda \bth^\star(\lambda) + R(\delta\bth,\lambda), \qquad
\|R(\delta\bth,\lambda)\|_2 \le C_\mathrm{nl} \|\delta\bth\|_2^2.
}
\end{align}

%--------------------------------------------------
\subsection{Explicit evaluation of the nonlinear constant $C_{\rm nl}$}
%--------------------------------------------------
For the final scaling, we need an explicit bound for the nonlinear remainder constant $C_{\rm nl}$ appearing in \eref{eq: tdvp bounds}.  Throughout, we consider the Pauli--rotation ansatz $|\psi(\bth)\rangle=\prod_{j=0}^{M-1} e^{-iP_j\theta_j}|0\rangle$ with $\|P_j\|_{\rm op}=1$.

We have to upper bound the following terms
\begin{equation}
C_{\rm nl} = \frac12 L_E \|\bG\|_{\rm op} + L_G \|\mathcal{H}\|_{\rm op},\nonumber
\end{equation}
where
\begin{align}
L_E &= \sup_{\bth\in B(\bth^\star,r)}
\|\nabla_\bth^3 E(\bth,\lambda)\|_{\rm op},\\
L_G &: \|G(\bth)-G(\bth^\star)\|_{\rm op}
\le L_G\|\bth-\bth^\star\|_2.
\end{align}
\subsubsection*{Third-derivative bound $L_E$}
From the commutator representation of third derivatives derived in \sref{sec: setup},
\begin{equation}
\partial_m\partial_k\partial_\ell E(\bth)=\langle\psi|[[\widetilde P_m,\widetilde P_k], [\widetilde P_\ell,H]]|\psi\rangle +\text{permutations},
\end{equation}
and using $\|\widetilde P_j\|_{\rm op}=1$ together with $\|[X,Y]\|_{\rm op}\le 2\|X\|_{\rm op}\|Y\|_{\rm op}$, each nested commutator term obeys
\begin{equation}
\big| \partial_m\partial_k\partial_\ell E \big| \le 8\|H\|_{\rm op}.
\end{equation}

The operator norm of the third-derivative tensor is defined as
\begin{equation}
\|\nabla_\bth^3 E\|_{\rm op}
=
\sup_{\|u\|_2=\|v\|_2=\|w\|_2=1}
\Big|
\sum_{m,k,\ell} u_m v_k w_\ell
\partial_m\partial_k\partial_\ell E
\Big|.
\end{equation}
Grouping the sum by the first index and using
$\|u\|_1\le \sqrt{M}\|u\|_2$ gives
\begin{equation}
\|\nabla_\bth^3 E\|_{\rm op}
\le \sqrt{M}
\max_m \|\nabla_m^3E\|_{\rm op}.
\end{equation}
With the bound
$\|\nabla_m^3E\|_{\rm op}\le 24\|H\|_{\rm op}M$
derived in \eref{eq: nabla^3 bound} we obtain the explicit constant
\begin{equation}
\boxed{
L_E \le 24\,\|H\|_{\rm op}\,M^{3/2}.
}
\label{eq:LE_bound}
\end{equation}

\subsubsection*{Lipschitz constant of the inverse metric}
To bound $L_G$ in Eq.~(S3.160) we control the Jacobian of $G=g^{-1}$.
For any $\theta,\theta'$ in a neighborhood $B$,
\[
\|G(\theta')-G(\theta)\|_{\rm op}
\le \sup_{\xi\in B}\Big\|\sum_{k=1}^M v_k \partial_k G(\xi)\Big\|_{\rm op}\,\|\theta'-\theta\|_2,
\]
and using $\|v\|_1\le \sqrt{M}\|v\|_2$ we obtain
\[
L_G \le \sqrt{M}\,\sup_{\theta\in B}\max_k \|\partial_k G(\theta)\|_{\rm op}.
\]
Differentiating $G(\theta)=g(\theta)^{-1}$ yields
$\partial_k G(\theta)=-G(\theta)(\partial_k g(\theta))G(\theta)$ and hence
\[
\|\partial_k G(\theta)\|_{\rm op}\le \|G(\theta)\|_{\rm op}^2\,\|\partial_k g(\theta)\|_{\rm op}.
\]
For the Pauli-rotation ansatz with $\|\widetilde P_j\|_{\rm op}=1$ the metric can be written as a covariance of
$\widetilde P_\mu$, and the identity $\partial_k\langle A\rangle=i\langle[\widetilde P_k,A]\rangle$
implies
\[
|\partial_k g_{\mu\nu}|\le \|[\widetilde P_k,\widetilde P_\mu\widetilde P_\nu]\|_{\rm op}
+\|[\widetilde P_k,\widetilde P_\mu]\|_{\rm op}|\langle\widetilde P_\nu\rangle|
+|\langle\widetilde P_\mu\rangle|\|[\widetilde P_k,\widetilde P_\nu]\|_{\rm op}
\le 6,
\]
so $\|\partial_k g(\theta)\|_{\rm op}\le 6M$.
Assuming $g(\theta)\succeq (\gamma/2)I$ on $B$, we have $\|G(\theta)\|_{\rm op}\le 2/\gamma$ and therefore
\[
\|\partial_k G(\theta)\|_{\rm op}\le (2/\gamma)^2(6M)=24M/\gamma^2,
\qquad
L_G \le \sqrt{M}\,24M/\gamma^2
= 24 M^{3/2}/\gamma^2.
\]

\subsubsection*{Final bound on $C_{\rm nl}$}
Using \lref{lem: smoothness}, the Hessian of the variational energy obeys $\|\mathcal{H}(\theta,\lambda)\|_{\mathrm{op}} =\|\nabla_\theta^2E(\theta,\lambda)\|_{\mathrm{op}}\le 4\|H(\lambda)\|_{\mathrm{op}}\,M$.
Therefore
\begin{align}
C_{\rm nl}&\le \frac12\left(24\|H\|_{\mathrm{op}}M^{3/2}\right)\frac{1}{\gamma} + \left(\frac{8M^{3/2}}{\gamma^2}\right)\|\mathcal{H}\|_{\mathrm{op}} \nonumber\\
&\le \frac{12}{\gamma}\|H\|_{\mathrm{op}}M^{3/2} + \frac{32}{\gamma^2}\|H\|_{\mathrm{op}}M^{5/2}\approx \frac{32}{\gamma^2}\|H\|_{\mathrm{op}}M^{5/2}.
\label{eq: cnl bound}
\end{align}

\subsection{Imaginary-time ground state following}
The following theorem is an imaginary time version of the theorem proven in~\cite{ZuEtAl25}.
\begin{theorem}[Imaginary-time ground state variational adiabatic theorem]
\label{thm:geo-tdvp-final}
Let $\bth(\tau)$ satisfy \eqref{eq:tdvp-flow}. Then
\begin{align}
\|\delta\bth(\tau)\|_2 \le \frac{D}{T \deltamin} (1 - e^{-\deltamin \tau}), 
\qquad \forall \tau \in [0, T].
\end{align}
\end{theorem}
\begin{proof}
Let
\[
\delta\bth(\tau) = \bth(\tau)-\bth^\star(\lambda(\tau)),
\qquad
u(\tau)=\|\delta\bth(\tau)\|_2 .
\]
From \eref{eq: tdvp reminder}, the deviation satisfies
\[
\dot{\delta\bth}
=
\bK(\lambda)\,\delta\bth
-\frac{1}{T}\partial_\lambda\bth^\star(\lambda)
+
\mathcal R(\delta\bth,\lambda),
\]
with
\(
\|\mathcal R(\delta\bth,\lambda)\|_2
\le
C_{\mathrm{nl}}\|\delta\bth\|_2^2
\).
For $u(\tau)>0$, differentiating the norm yields
\[
\frac{d}{d\tau}u
=
\frac{\langle \delta\bth,\dot{\delta\bth}\rangle}{\|\delta\bth\|_2}.
\]
Substituting the evolution equation gives
\begin{align}
\frac{d}{d\tau}u
&=
\frac{\langle \delta\bth, \bK(\lambda)\delta\bth\rangle}{\|\delta\bth\|_2}
-
\frac{1}{T}
\frac{\langle \delta\bth,\partial_\lambda\bth^\star\rangle}{\|\delta\bth\|_2}
+
\frac{\langle \delta\bth,\mathcal R(\delta\bth,\lambda)\rangle}{\|\delta\bth\|_2}.
\label{eq:norm-derivative}
\end{align}
\medskip
By \aref{supp: ass: geometry}, the linearized TDVP generator
\(
\bK(\lambda)=-\bG(\bth^\star)\mathcal{H}(\lambda)
\)
is strictly dissipative on the subspace orthogonal to gauge directions, i.e.,
\[
\label{eq: K bound}
\langle x,\bK(\lambda)x\rangle
\le
-\deltamin\,\|x\|_2^2
\qquad
\forall x \perp \text{gauge}.
\]
Since $\delta\bth$ is defined modulo gauge equivalence, this yields
\[
\frac{\langle \delta\bth, \bK(\lambda)\delta\bth\rangle}{\|\delta\bth\|_2}
\le
-\deltamin\,u.
\]
\medskip
Using Cauchy--Schwarz and the drift bound \lref{lem:drift-bound},
\[
\frac{1}{T}
\frac{|\langle \delta\bth,\partial_\lambda\bth^\star\rangle|}{\|\delta\bth\|_2}
\le
\frac{1}{T}\|\partial_\lambda\bth^\star\|_2
\le
\frac{D}{T}.
\]
Similarly, using the quadratic bound on the nonlinear remainder,
\[
\frac{|\langle \delta\bth,\mathcal R(\delta\bth,\lambda)\rangle|}{\|\delta\bth\|_2}
\le
\|\mathcal R(\delta\bth,\lambda)\|_2
\le
C_{\mathrm{nl}}u^2.
\]
\medskip
Combining the above estimates in Eq.~\eqref{eq:norm-derivative}, we obtain
\[
\frac{d}{d\tau}u
\le
-\deltamin\,u
+
\frac{D}{T}
+
C_{\mathrm{nl}}u^2.
\]
Since $u(0)=0$ and the solution remains $O(1/T)$ for finite $\tau$, the quadratic
term is higher order in $1/T$ and can be discarded for an upper bound, yielding
\[
\frac{d}{d\tau}u
\le
-\deltamin\,u
+
\frac{D}{T}.
\]
\medskip
The next step provides a self-consistent justification of the approximation by dropping the quadratic term.

Solving this differential inequality with $u(0)=0$ gives
\[
u(\tau)
\le
\frac{D}{T\deltamin\,}
\left(1-e^{-\deltamin\,\tau}\right),
\qquad
\tau\in[0,T].
\]
\end{proof}
At this stage, we still have the optimal adiabatic complexity $1/\deltamin^2$, since $D=\mathcal{O}(1/\deltamin)$. In the following section, we see that discrete updates introduce an additional $1/\deltamin$ due to stability, analogous to the condition that the optimised parameters should remain in the PŁ region.

% ======================================================
\subsection{Numerical stability and gradient-update complexity}
% ======================================================

\subsubsection*{Discrete-time TDVP update}
We discretize the imaginary-time TDVP flow
\begin{align}
\frac{d\bth}{d\tau} = -\bG(\bth)\nabla_\bth E(\bth,\lambda),
\end{align}
with step size $\eta>0$ and linear schedule $\lambda_n = n \eta / T$, $n=0,1,\dots,\nupdate-1$, $\nupdate=T/\eta$:
\begin{align}
\bth_{n+1} = \bth_n - \eta\, \bG(\bth_n)\nabla_\bth E(\bth_n,\lambda_n).
\label{eq:tdvp-discrete-final}
\end{align}
Let the deviation from the instantaneous minimizer be
\begin{align}
\delta\bth_n = \bth_n - \bth^\star(\lambda_n),
\end{align}
where $\bth^\star(\lambda)$ is the exact variational ground state for each $\lambda$.

\subsubsection*{Linearization and nonlinear bounds}
Expand the gradient and metric:
\begin{align}
\nabla_\bth E(\bth_n,\lambda_n) &= \mathcal{H}(\lambda_n)\delta\bth_n + R_n, &  \|R_n\|_2 \le \frac{1}{2} L_E \|\delta\bth_n\|_2^2,  \label{eq:grad-expand-final}\\
\bG(\bth_n) &= \bG(\bth^\star(\lambda_n)) + \Delta \bG_n, &  \|\Delta \bG_n\|_{\rm op} \le L_G \|\delta\bth_n\|_2. \label{eq:metric-expand-final}
\end{align}
Then the discrete deviation satisfies
\begin{align}
\delta\bth_{n+1} = (I - \eta \bK_n) \delta\bth_n - (\bth^\star(\lambda_{n+1}) - \bth^\star(\lambda_n)) - \eta (\Delta \bG_n \mathcal{H} \delta\bth_n + (\bG + \Delta \bG_n) R_n).
\label{eq: discrete recursion}
\end{align}
Using the submultiplicativity of operator norms together with
\eqref{eq:grad-expand-final}–\eqref{eq:metric-expand-final}, we estimate
\begin{align}
\|\Delta \bG_n \mathcal{H}(\lambda_n)\delta\bth_n\|_2
&\le \|\Delta \bG_n\|_{\mathrm{op}}\|\mathcal{H}\|_{\mathrm{op}}\|\delta\bth_n\|_2
\le L_G\|\mathcal{H}\|_{\mathrm{op}}\|\delta\bth_n\|_2^2,\\
\|(\bG(\bth_n))R_n\|_2
&\le \|\bG(\bth_n)\|_{\mathrm{op}}\|R_n\|_2 \le \|\bG\|_{\mathrm{op}}\tfrac12 L_E\|\delta\bth_n\|_2^2,
\end{align}
Combining both contributions yields
\begin{align}
\|\bG(\bth_n)\nabla_\bth E(\bth_n,\lambda_n) - \bg(\bth^\star)\mathcal{H}(\lambda_n)\delta\bth_n\|_2 \le C_{\mathrm{nl}}\|\delta\bth_n\|_2^2,
\label{eq:nonlinear-final}
\end{align}
where $C_{\rm nl}$ is the same as in the continuous case \eref{eq: tdvp bounds}. Substituting \eqref{eq: K bound}, \eqref{eq:nonlinear-final}, and \lref{lem:drift-bound} into \eqref{eq: discrete recursion} and applying the triangle inequality, we obtain
\begin{align}
\boxed{\|\delta\bth_{n+1}\|_2 \le (1-\eta\deltamin\,)\|\delta\bth_n\|_2 + b + c\|\delta\bth_n\|_2^2}, 
\label{eq:discrete tdvp}
\end{align}
where $c=\eta C_{\mathrm{nl}}$.

\subsubsection*{Global discrete tracking bound}
\begin{theorem}[Uniform discrete tracking bound]
Let $\delta\bth_n=\bth_n-\bth^\star(\lambda_n)$ satisfy the discrete TDVP update with $\delta\bth^\star=0$. Assume that the step size satisfies
\begin{align}
0<\eta\le\frac{1}{2\|H\|_{\mathrm{op}}},
\label{eq:eta-thm2}
\end{align}
and that the total evolution time $T$ satisfies
\begin{align}
T \ge \frac{4 C_{\mathrm{nl}} D}{\deltamin\,^2}.
\label{eq:T-thm2}
\end{align}
Define
\begin{align}
A = \frac{2 D}{T\deltamin\,}.
\label{eq:A-def}
\end{align}
Then for all $n=0,1,\dots,\nupdate$,
\begin{align}
\|\delta\bth_n\|_2 \le A.
\label{eq:uniform-bound}
\end{align}
In particular, the iterates remain inside the locality radius where the perturbations in \eref{eq:grad-expand-final} and \eref{eq:metric-expand-final} remain valid.
\end{theorem}
\begin{remark} 
Due to stability, the time $T$ has to scale as $1/\deltamin^3$, whereas the error scales as $1/T\deltamin^2$.
\end{remark}

\begin{proof}
Define
\[
a_n = \|\delta\bth_n\|_2.
\]
By \eref{eq:discrete tdvp}, the sequence $\{a_n\}_{n\ge0}$ satisfies the deterministic recursion
\begin{align}
a_{n+1}
\le
(1-\eta\deltamin\,)a_n
+
b
+
c a_n^2,
\label{eq:recursion}
\end{align}
where
\[
b = \eta\frac{D}{T},
\qquad
c = \eta C_{\mathrm{nl}}.
\]
We prove by induction that
\[
a_n \le A
\quad\text{for all }n\ge0,
\]
with $A$ defined in \eqref{eq:A-def}. By assumption, $\delta\bth^\star=0$, hence
\[
a_0 = 0 \le A.
\]
Assume $a_n \le A$ for some $n\ge0$. We show that $a_{n+1}\le A$. Using \eqref{eq:recursion} and the induction hypothesis,
\begin{align}
a_{n+1} &\le (1-\eta\deltamin\,)A + b + c A^2.
\label{eq:induction-bound}
\end{align}
Thus, it suffices to verify that
\begin{align}
(1-\eta\deltamin\,)A + b + cA^2 \le A.
\label{eq:suffices}
\end{align}
Rearranging \eqref{eq:suffices} gives the quadratic inequality
\begin{align}
cA^2 - \eta\deltamin\,A + b \le 0.
\label{eq:quad-ineq}
\end{align}
Consider the quadratic polynomial
\[
p(a)=c a^2-\eta\deltamin\,a+b.
\]
Assume the discriminant is nonnegative,
\begin{equation}
\mathrm{Disc}=\eta^2\deltamin\,^2-4bc\ge0.
\label{eq:disc_condition}
\end{equation}
Then $p$ has two real roots
\[
A_{\pm}=\frac{\eta\deltamin\,\pm\sqrt{\mathrm{Disc}}}{2c}, \qquad 0<A_- \le A_+.
\]
Moreover, on $[0,A_-]$ we have $1-\eta\deltamin\,+2ca\ge 0$. Hence, for any $a\in[0,A_-]$,
\[
(1-\eta\deltamin\,)a + b + ca^2 < A_-.
\]
Since $a_0=0\in[0,A_-]$, we obtain by induction that
\[
a_n\le A_- \qquad \text{for all } n=0,1,\dots,\nupdate.
\]
Thus, the \emph{guaranteed tracking region} can be chosen as the smaller root
\begin{equation}
A=A_-=\frac{\eta\deltamin\,-\sqrt{\eta^2\deltamin\,^2-4bc}}{2c}.
\label{eq:Aminus_exact}
\end{equation}
The smaller root can be rewritten as
\[
A_-=
\frac{\eta\deltamin\,-\sqrt{\eta^2\deltamin\,^2-4bc}}{2c}
=
\frac{2b}{\eta\deltamin\,+\sqrt{\eta^2\deltamin\,^2-4bc}},
\]
where the second equality follows by multiplying the numerator and denominator by
$\eta\deltamin\,+\sqrt{\eta^2\deltamin\,^2-4bc}$.
Since $\sqrt{\eta^2\deltamin\,^2-4bc}\ge 0$, we obtain the upper bound
\[
A_- \le \frac{2b}{\eta\deltamin\,}.
\]
Using $b=\eta D/T$, this yields the sufficient choice
\[
A \le \frac{2D}{T\deltamin\,},
\]
which coincides with \eqref{eq:A-def}. The discriminant condition \eqref{eq:disc_condition} becomes
\[
\eta^2\deltamin\,^2 \ge 4bc
\quad\Longleftrightarrow\quad
\deltamin\,^2 \ge 4C_{\mathrm{nl}}\frac{D}{T},
\]
i.e.
\[
T \ge \frac{4C_{\mathrm{nl}}D}{\deltamin\,^2},
\]
which is exactly the hypothesis \eqref{eq:T-thm2}.
By induction,
\[
a_n=\|\delta\bth_n\|_2 \le A
\quad\text{for all }n=0,1,\dots,\nupdate.
\]
Finally, using \eqref{eq:T-thm2}
\[
A = \frac{2D}{T\deltamin\,}
\le
\frac{\deltamin\,}{2C_{\mathrm{nl}}}
\]
Hence, all iterates remain inside the region where \eref{eq:discrete tdvp} applies.
\end{proof}

\subsubsection*{Gradient-update complexity}
To achieve tracking error $\|\delta\bth\|_2 \le \varepsilon$, one must satisfy
\begin{align}
T \ge \max \Big\{ \frac{4 C_{\rm nl} D}{\deltamin\,^2}, \frac{2 D}{\varepsilon \deltamin\,} \Big\},
\end{align}
with step size $\eta = 1/(2\|H\|_{\rm op})$. Therefore, the number of gradient updates is
\begin{align}
\nupdate = \frac{T}{\eta} \ge 4 \|H\|_{\rm op} \frac{D}{\deltamin\,} \max \Big\{ \frac{C_{\rm nl}}{\deltamin\,}, \frac{1}{\varepsilon} \Big\}.
\end{align}

Using $D=\frac{\sqrt{M}\,\|\partial_\lambda H\|_{\mathrm{op}}}{\gamma\,\Delta_{\min}}$ and the dominant contribution
$C_{\rm nl}\simeq \frac{32}{\gamma^2}\|H\|_{\mathrm{op}}M^{5/2}$, \eref{eq: cnl bound} yields the approximate scaling
\begin{equation}
\boxed{N_{\rm update} \simeq\ 128\frac{M^3\,\|H\|_{\mathrm{op}}^2\,\|H_\text{f}-H_\text{i}\|_{\mathrm{op}}}{\gamma^{3}\,\Delta_{\min}^{3}}}\,,
\label{eq:Nupdate_TDVP_approx}
\end{equation}
up to subleading terms in $M$ and universal numerical constants.

% ======================================================
\subsection{Comparison of P\L{} and TDVP scalings.}
% ======================================================
The three analyses presented above provide complementary perspectives on the same tracking dynamics.  Both P\L{} constructions yield the same overall update complexity  $N_{\rm updates}\propto \Delta_{\min}^{-3}$,  but distribute the cost differently:  P\L{} \texttt{option~1} employs comparatively large adiabatic steps $\delta\lambda\propto \Delta_{\min}^{2}$ together with many optimization  steps per slice $K\propto \Delta_{\min}^{-1}$, whereas P\L{} \texttt{option~2} keeps $K=\mathcal{O}(1)$ and compensates  by refining the discretization to $\delta\lambda\propto \Delta_{\min}^{3}$. The TDVP derivation instead starts from a continuous-time imaginary-time flow, which exhibits the expected adiabatic scaling $T\propto \Delta_{\min}^{-2}$.  For explicit discretizations, an additional factor $\Delta_{\min}^{-1}$ appears due to the stability constraint on the update size, reflecting the stiffness of the gradient flow near small gaps.

Implicit (proximal-point) discretizations provide a complementary interpretation.
While such schemes remove the explicit stability restriction on the step size and allow larger adiabatic increments~\cite{HaWa96}, each proximal update corresponds to solving a strongly convex subproblem whose contraction rate scales as $\mu\sim\gamma\Delta_{\min}$.  Consequently, the additional $\Delta_{\min}^{-1}$ factor reappears through the inner optimization effort, making proximal TDVP closely analogous to P\L{} \texttt{option~1}~\cite{KaNuSc20}.
From a physical perspective, this behaviour reflects the intrinsic adiabatic curvature of the variational manifold: as the spectral gap narrows, the local contraction rate governing relaxation towards the instantaneous ground-state branch decreases proportionally to $\Delta_{\min}$, so that any local first-order tracking scheme---explicit or implicit---requires $\mathcal{O}(\Delta_{\min}^{-1})$ relaxation steps per adiabatic time scale. Thus, the extra gap dependence is not merely a numerical artefact of explicit integration, but a manifestation of the geometric slowdown near small gaps, and all viewpoints consistently lead to the same asymptotic update scaling while illuminating different allocations of 
computational effort.

% ======================================================
\section{Absence of barren plateaus}
% ======================================================
In this section, we present a proof of the absence of barren plateaus, i.e., gradients that decrease exponentially with the system size, when we are exploring the energy landscape close to a minimum.
The proof can be explained in the following way: we write the energy cost function in Taylor form around the minimum $\bth^*$, and choose a small-enough radius $r$ such that we can approximate the energy as a quadratic form up to error $\epsilon_{\mathrm{Q}}$.
In this approximation, we show that the variance of the loss function does not decay exponentially with system size.
We strees that we are proving a stronger condition than the presence of gradients: we show the region where the energy is approximately quadratic.

\begin{theorem}[Non-vanishing variance of the energy close to the minimum]
    Let $\ket{\psi(\bth)}$ be the variational ansatz with $M$ parameters, and let $\bth^*$ be the minimum of the the energy function $E(\bth)=\bra{\psi(\bth)}H\ket{\psi(\bth)}$.
    Suppose the perturbations $\delta\bm{\theta}$ are independently identically distributed variables drawn from the normal distribution:
    \begin{align}
        \delta\theta_j\sim N\left(0, \frac{\epsilon_{\mathrm{Q}}}{12 \norm{H}_{\mathrm{op}} M^{3/2}}\right).
    \end{align}
    Then, the energy variance is polynomial in the number of parameters $M$, i.e.:
    \begin{align}
    \Var_{\delta\bm{\theta}}\Big[E(\bth^*+\delta\bm{\theta})\Big]\geq \frac{\Delta^6_{\min}\epsilon_{\mathrm{Q}}^4}{12^4\norm{H}_{\mathrm{op}}^4M^7}\left(\sum_k 1-\abs{\bra{\hat{0}}\widetilde{P}_k\ket{\hat{0}}}^2\right)^2.
    \end{align}
    with $\epsilon_{\mathrm{Q}}\in(0,1)$.
\end{theorem}

\begin{proof}
    We start by determining the radius for which $E(\bth^*+\delta\bm{\theta})$ can be approximated as a quadratic form, i.e.:
    \begin{align}
    E(\bm{\theta}^*+\delta\bm{\theta})=E(\bm{\theta}^*)+\frac{1}{2}\delta\bm{\theta}^T\mH(\bm{\theta}^*)\delta\bm{\theta} +\frac{1}{6}\sum_{ijk}T_{ijk}(\bm{\theta})\delta\theta^3\approx E(\bm{\theta}^*)+\frac{1}{2}\delta\bm{\theta}^T\mH(\bm{\theta}^*)\delta\bm{\theta},
    \end{align}
    which leads to the condition on the perturbation $\delta\theta$:
    \begin{align}
        \delta\theta\leq3\epsilon_{\mathrm{Q}}\frac{\norm{\mH(\bm{\theta}^*)}_{\mathrm{op}}}{\max_{\bm{\theta}\in( \bm{\theta}^*+\delta\bm{\theta})}\norm{T(\bm{\theta})}_{\mathrm{op}}}.
    \end{align}
    To have a rigorous bound, we first lower-bound the numerator and then upper-bound the denominator.
    For the numerator, we use Lemma~\ref{lem: hess lower bound} to bound $\norm{\mH}_{\mathrm{op}}$:
    \begin{align}
    \norm{\mH}_{\mathrm{op}} & \geq 2\gamma\Delta_{\min{}},
    \end{align}
    and for the denominator we recall Eq.~\eqref{eq:LE_bound}: 
    \begin{align}
        \norm{T}_{\mathrm{op}}\leq 24M^{3/2}\norm{H}_{\mathrm{op}}.
    \end{align}
    The radius $\delta\theta_{\mathrm{Q}}$ where we can approximate the energy as a quadratic form reads:
    \begin{align}\label{eq:radius}
        \delta\theta \leq
        \delta\theta_{\mathrm{Q}}= \epsilon_{\mathrm{Q}}\frac{\gamma\Delta_{\min}}{12M^{3/2}\norm{H}_{\mathrm{op}}}.
    \end{align}
    For $\delta\theta\leq\delta\theta_{\mathrm{Q}}$, we can write the energy as:
    \begin{align}
    E(\bm{\theta}^*+\delta\bm{\theta})\approx E(\bm{\theta}^*)+\frac{1}{2}\delta\bm{\theta}^T\mH(\bm{\theta}^*)\delta\bm{\theta},
    \end{align}
    and the variance of the energy becomes:
    \begin{align}
        \Var_{\delta\bm{\theta}}\Big[E(\bm{\theta}^*+\delta\bm{\theta}) \Big]\approx \frac{1}{2}\Var_{\delta\bm{\theta}}\Big[\delta\bm{\theta}^T\mH(\bm{\theta}^*)\delta\bm{\theta}\Big].
    \end{align}
    When each i.i.d. random variable $\delta\theta$ is drawn from a normal distribution of mean $\mu=0$ and standard deviation $\sigma=\delta\theta_{\mathrm{Q}}$ the variance of the quadratic form is well known~\cite{MaPr92}:
    \begin{align}
        \Var_{\delta\bm{\theta}}\Big[\delta\bm{\theta}^T\mH(\bm{\theta}^*)\delta\bm{\theta}\Big]=\frac{\delta\theta_{\mathrm{Q}}^4}{2}\norm{\mH}^2_F\geq\frac{\delta\theta_{\mathrm{Q}}^4}{2M}\Tr{\mH}^2.
    \end{align}
    We focus on the diagonal element of the Hessian in spectral form, where $\ket{\hat{n}}$ is the $n$-th eigenvector of the Hamiltonian $H$:
    \begin{align}
    \mH_{kk}(\bm{\theta}^*)&=2\sum_{n\geq1} (E_i-E_0)\abs{ \bra{\hat{0}}\widetilde{P}_k\ket{\hat{n}}}^2\geq 2(E_1-E_0)\sum_{n\geq1}\abs{\bra{\hat{0}}\widetilde{P}_k\ket{\hat{n}}}^2
    \\
    &=2\Delta_{10}\sum_{n\geq1}\bra{\hat{0}}\widetilde{P}_k\ket{\hat{n}}\bra{\hat{n}}\widetilde{P}_k\ket{\hat{0}}=2\Delta_{10}\left( \sum_{n\geq0}\bra{\hat{0}}\widetilde{P}_k\ket{\hat{n}}\bra{\hat{n}}\widetilde{P}_k\ket{\hat{0}} - \abs{\bra{\hat{0}}\widetilde{P}_k\ket{\hat{0}}}^2\right) \\
    &= 2\Delta_{10}\left( \bra{\hat{0}}\widetilde{P}_k^2\ket{\hat{0}} - \abs{\bra{\hat{0}}\widetilde{P}_k\ket{\hat{0}}}^2\right)=2\Delta_{10}\left( 1-\abs{\bra{\hat{0}}\widetilde{P}_k\ket{\hat{0}}}^2 \right)\geq 2\Delta_{\min}\left( 1-\abs{\bra{\hat{0}}\widetilde{P}_k\ket{\hat{0}}}^2 \right),
\end{align}
    where $\Delta_{\min}$ is the minimum gap across the adiabatic path.
    Thus, we obtain:
    \begin{align}
        \frac{1}{2}\Var_{\delta\bm{\theta}}\Big[\delta\bm{\theta}^T\mH(\bm{\theta}^*)\delta_{\min}\bm{\theta}\Big]\geq\frac{\delta\theta_{\mathrm{Q}}^4}{4M}4\Delta^2\left(\sum_k 1-\abs{\bra{\hat{0}}\widetilde{P}_k\ket{\hat{0}}}^2\right)^2=\frac{\Delta_{\min}^6}{12^4\norm{H}_{\mathrm{op}}^4M^7}\left(\sum_k 1-\abs{\bra{\hat{0}}\widetilde{P}_k\ket{\hat{0}}}^2\right)^2.
    \end{align}
    Note that in the best case scenation, when $\abs{\bra{\hat{0}}\widetilde{P}_k\ket{\hat{0}}}\approx$ we can obtain:
    \begin{align}
        \Var_{\delta\bm{\theta}}\Big[E(\bm{\theta}^*+\delta\bm{\theta}) \Big]\approx\frac{\epsilon_{\mathrm{Q}}^4\Delta^6_{\min{}}}{12^4\norm{H}_{\mathrm{op}}^4M^5}
    \end{align}
\end{proof}

% ======================================================
\section{Proof of Theorem 2: Standard-deviation-based verification}\label{sec:verification}
% ======================================================
In this section, we introduce a \emph{verification layer} which certifies, at each adiabatic step, that the variational state lies on the correct (ground-state) spectral branch. The verification procedure is entirely based on measurements of the energy standard deviation and is logically independent of the optimization method used to update the variational parameters. Throughout this section, the standard deviation is used solely as a \emph{diagnostic observable}. It does not drive the optimization but serves to certify eigen-branch identity and, once the branch is identified, to quantify the overlap with the corresponding eigenstate.

% ======================================================
\subsection{Setup, assumptions, and proof roadmap}
% ======================================================
To make the presentation easier, we extend our setup and assumptions from \sref{sec: setup}. We define the spectral decomposition
\[
H(\lambda) = \sum_{j\ge 0} E_j(\lambda)\, \Pi_j(\lambda),
\qquad
E_0(\lambda) < E_1(\lambda) \le E_2(\lambda) \le \cdots ,
\]
where $\Pi_j(\lambda)$ denotes a projector to $j-$th eigenstate. For any normalized state $\ket{\psi}$ and Hermitian operator $A$, we define
\begin{align}
\Std_\psi(A)
&=  \sqrt{\bra{\psi} A^2 \ket{\psi} - \bra{\psi} A\ket{\psi}^2}, \\
E_\psi(\lambda)
&= \bra{\psi} H(\lambda) \ket{\psi}, \quad \mbox{and}\quad  \Std_\psi(\lambda)=\Std_\psi(H(\lambda)).
\end{align}
In addition, we introduce a new assumption.
\begin{assumption}[Uniform gap \emph{to the tracked branch}]
\label{ass:global_gap_ver}
Let $j_\star$ denote the eigen-branch. Assume there exists $\deltaminj>0$ such that, for all $\lambda\in[0,1]$,
\begin{equation}
\min_{j\neq j_\star} \big|E_j(\lambda)-E_{j_\star}(\lambda)\big|
\ge
\deltaminj.
\label{eq:tracked_gap}
\end{equation}
\end{assumption}
For the main theorem, we use $j_\star=0$ (which reduces Assumption 4 to Assumption 1), but we state some lemmas more generally. 

\medskip
\noindent
\texttt{Proof roadmap:}
The goal of this section is to turn \emph{measured energy standard deviation} into a \emph{runtime verification} that the algorithm remains on the intended eigen-branch (in particular, the ground-state branch) throughout the adiabatic evolution, and to quantify the resulting fidelity. The proof of \texttt{Theorem~2} in the main text is obtained in several steps:

\begin{enumerate}
\item \textbf{Eigen-branch identification from standard deviation.}
First, we show that, for any state $\ket{\psi}$ at a fixed $\lambda$, the mean energy $E_\psi(\lambda)$ must lie within one standard deviation of \emph{some} eigenvalue $E_j(\lambda)$. Moreover, if the measured standard deviation is smaller than half the uniform branch gap, then this index is \emph{unique}. This is \lref{lem:variance_branch}.

\item \textbf{From identification to fidelity.}
Once the relevant branch $j_\star$ is uniquely identified, we convert the same standard deviation value into a quantitative lower bound on the overlap $\bra{\psi}\Pi_{j_\star}(\lambda)\ket{\psi}$. This is Lemma~\ref{lem:var_to_fid_branch} and its specialization to the ground state in \cref{cor:ground_fidelity}. In our final theorem, we use $j_\star=0$.

\item \textbf{Warm-start verification for linear schedules.}
We then analyze the canonical warm-start state $\ket{0(\lambda)}$ when the schedule advances to $\lambda^+=\lambda+\delta\lambda$. For a linear interpolation $H(\lambda)$, the energy standard deviation of the warm start with respect to the \emph{new} Hamiltonian is \emph{exactly quadratic} in $\delta\lambda$, yielding an explicit step-size condition that guarantees $\Std_{0(\lambda)}(H(\lambda^+))<\deltamin\,/2$. This is Lemma~\ref{lem:warm_start_exact} and the subsequent step-size lemma.

\item \textbf{Warm-start verification for general states.}
To decouple verification from the assumption of an exact eigenstate warm start, we prove a one-step \emph{propagation} inequality:
\[
\Std_\psi(\lambda^+)\le\Std_\psi(\lambda)+|\delta\lambda|\,\Std_\psi(H_\text{f}-H_\text{i}),
\]
based on a covariance bound (Cauchy--Schwarz). This yields a directly checkable sufficient condition for unique branch identification and (constant) fidelity at $\lambda^+$ from measurements at $\lambda$. This is done in Lemmas~\ref{lem:covariance_bound}--\ref{lem:variance_propagation} and Corollary~\ref{cor:verification_condition}.

\item \textbf{Coupling verification to PŁ tracking.}
Finally, we combine the verification certificate with the PL-based contraction guarantee from the optimization analysis: if the warm start is certified to lie on the round branch at $\lambda^+$ and the PŁ region drifts continuously, then (i) the same parameters remain inside the PŁ region at $\lambda^+$ and (ii) subsequent gradient steps ontract toward $\bth^\star(\lambda^+)$. This yields a \emph{self-verified} adiabatic update rule. This combination is formalized in \tref{thm:verification_pl_tracking}.

\end{enumerate}

% ======================================================
\subsection{Lemmas and corollaries}
% ======================================================

\subsubsection*{Variance as an eigen-branch identifier}

\begin{lemma}[Standard deviation identifies a unique ground state]
\label{lem:variance_branch}
For any $\lambda$ and any normalized state $\ket{\psi}$, there exists an index
$j$ such that
\begin{equation}
\big| E_\psi(\lambda) - E_j(\lambda) \big|
\le \Std_\psi(\lambda) .
\end{equation}
If $\Std_\psi(\lambda) < \deltamin\,/2$, then this index $j$ is unique.
\end{lemma}

\begin{proof}
Let $p_j = \bra{\psi} \Pi_j(\lambda) \ket{\psi}$.
Then
\[
\Std_\psi(\lambda)^2
=
\sum_{j\ge 0} p_j \big(E_j(\lambda) - E_\psi(\lambda)\big)^2 .
\]
If $|E_j - E_\psi| > \Std_\psi$ for all $j$, then
\[
\Std_\psi^2
>
\sum_j p_j \Std_\psi^2
= \Std_\psi^2,
\]
is a contradiction. Hence, at least one index $j$ satisfies the bound. If two distinct indices $j\neq k$ satisfy $|E_{j,k}-E_\psi|\le \Std_\psi$, then
\[
|E_j - E_k|
\le |E_j - E_\psi| + |E_k - E_\psi|
\le 2\Std_\psi
\].
If $\Std_\psi < \deltamin\,/2$ then the two eigenbranches $j,k$ satisfy:
\[
|E_j - E_k|<\deltamin\,
\]
contradicting Assumption~\ref{ass:global_gap_ver} (assuming additionally that the gap also holds for $j-$th eigenstate, i.e. $j=j_\star$).
\end{proof}

\subsubsection*{Fidelity certification for the identified eigen-branch}

\begin{lemma}[Standard deviation-to-fidelity bound for the identified branch]
\label{lem:var_to_fid_branch}
Fix $\lambda$ and a normalized state $\ket{\psi}$.
Assume $\Std_\psi(\lambda) < \deltamin\,/2$ and let $j_\star$ be the unique
index from \lref{lem:variance_branch}, i.e.
\[
|E_\psi(\lambda) - E_{j_\star}(\lambda)| \le \Std_\psi(\lambda) .
\]
Then
\begin{equation}
1 - \bra{\psi}\Pi_{j_\star}(\lambda)\ket{\psi}
\le
\frac{\Std_\psi(\lambda)^2}
{\big(\deltamin\, - \Std_\psi(\lambda)\big)^2}.
\label{eq:branch_fidelity}
\end{equation}
\end{lemma}

\begin{proof}
Expand $\ket{\psi}$ in the eigenbasis of $H(\lambda)$:
$\ket{\psi} = \sum_j \alpha_j \ket{E_j(\lambda)}$ with
$p_j = |\alpha_j|^2=\bra{\psi}\Pi_j\ket{\psi}$.
Then
\[
\Std_\psi(\lambda)^2
=
\sum_j p_j \big(E_j(\lambda) - E_\psi(\lambda)\big)^2 .
\]
Split the sum into the identified branch $j_*$ and its complement:
\[
\Std_\psi(\lambda)^2
=
p_{j_\star}\big(E_{j_\star}-E_\psi\big)^2
+
\sum_{j\neq j_\star} p_j\big(E_j-E_\psi\big)^2
\ge
\sum_{j\neq j_\star} p_j\big(E_j-E_\psi\big)^2,
\]
where we used the fact that each term is positive. For any $j\neq j_\star$,
\[
|E_j - E_\psi|
\ge
|E_j - E_{j_\star}| - |E_{j_\star} - E_\psi|
\ge
\deltamin\, - \sqrt{V_\psi(\lambda)},
\]
where we used Assumption~\ref{ass:global_gap_ver} and the definition of $j_\star$.
Therefore,
\[
\Std_\psi(\lambda)^2
\ge
\sum_{j\neq j_\star} p_j
\big(\deltamin\, - \Std_\psi(\lambda)\big)^2
=
\big(1 - p_{j_\star}\big)
\big(\deltamin\, - \Std_\psi(\lambda)\big)^2.
\]
Rearranging yields~\eqref{eq:branch_fidelity}.
\end{proof}

\begin{corollary}[Ground-state fidelity once the branch is known]
\label{cor:ground_fidelity}
Under Assumption~\ref{ass:global_gap_ver}, suppose that the unique index $j_\star$ in \lref{lem:variance_branch} equals $0$, i.e., we consider the ground state. If $\Std_\psi(\lambda) \le \deltamin\,/4$, then
\[
\bra{\psi}\Pi_0(\lambda)\ket{\psi}
\ge
\frac{8}{9}.
\]
\end{corollary}
\begin{proof}
Apply \lref{lem:var_to_fid_branch} with $j_\star = 0$. If $\Std_\psi \le \deltamin\,/4$, then $\deltamin\, - \Std_\psi \ge 3\deltamin\,/4$, giving the stated bound.
\end{proof}
We stress that $\deltamin\,/4$ is an arbitrary value and any $\Std<\deltamin\,/2$ would be feasible.

\subsubsection*{Exact warm-start variance for linear schedules}

\begin{lemma}[Exact warm-start standard deviation]
\label{lem:warm_start_exact}
Let $\ket{0(\lambda)}$ denote the ground state of $H(\lambda)$.
Then for any $\delta\lambda$,
\begin{equation}
\operatorname{\Std}_{0(\lambda)}\!\big(H(\lambda+\delta\lambda)\big)^2
=
\delta\lambda^2\,
\operatorname{\Std}_{0(\lambda)}\!\big(H_{\mathrm f}-H_{\mathrm i}\big)^2.
\end{equation}
\end{lemma}

\begin{proof}
Using
$H(\lambda+\delta\lambda)
=
H(\lambda) + \delta\lambda(H_{\mathrm f}-H_{\mathrm i})$
and
$H(\lambda)\ket{0(\lambda)} = E_0(\lambda)\ket{0(\lambda)}$,
all zeroth- and first-order contributions cancel in the variance expansion,
leaving only the quadratic term.
\end{proof}

\begin{lemma}[Verification step-size bound]
\label{lem:vericication_step}
If
\[
|\delta\lambda| < \frac{\deltamin\,} {2\operatorname{\Std}_{0(\lambda)}(H_{\mathrm f}-H_{\mathrm i})},
\]
then
\[
\operatorname{\Std}_{0(\lambda)}\!\big(H(\lambda+\delta\lambda)\big)<\frac{\deltamin\,}{2}.
\]
Consequently, the warm-start state $\ket{0(\lambda)}$ has overlap at least $8/9$
with the unique eigen-branch of $H(\lambda+\delta\lambda)$ identified by
\lref{lem:variance_branch}.
If this branch is the ground branch, then the overlap with the actual ground state
is at least $8/9$.
\end{lemma}

\begin{proof}
The standard deviation bound follows directly from \lref{lem:warm_start_exact}. Since $\sqrt{V} < \deltamin\,/2$, \lref{lem:variance_branch} and~\lref{lem:var_to_fid_branch} apply, yielding the stated fidelity bounds.
\end{proof}

\subsubsection*{Standard deviation propagation for a general warm start}

\begin{lemma}[Covariance bound]
\label{lem:covariance_bound}
For any Hermitian operators $A,B$ and any normalized state $\ket{\psi}$,
\[
\big|\mathrm{Cov}_\psi(A,B)\big|=
\big|
\bra{\psi} AB \ket{\psi}
-
\bra{\psi} A \ket{\psi}
\bra{\psi} B \ket{\psi}
\big|
\le
\operatorname{\Std}_\psi(A)\operatorname{\Std}_\psi(B) .
\]
\end{lemma}

\begin{proof}
Let
\[
\bar A = \bra{\psi}A\ket{\psi},\qquad \bar B = \bra{\psi}B\ket{\psi},
\]
and define the centered (Hermitian) operators
\[
\widetilde A = A-\bar A\,\mathbb I,\qquad \widetilde B = B-\bar B\,\mathbb I.
\]
Then
\begin{align}
\bra{\psi}AB\ket{\psi}-\bra{\psi}A\ket{\psi}\bra{\psi}B\ket{\psi}
&=
\bra{\psi}(A-\bar A\mathbb I)(B-\bar B\mathbb I)\ket{\psi} \notag\\
&=
\bra{\psi}\widetilde A\,\widetilde B\ket{\psi}.
\label{eq:cov_centered}
\end{align}
Now set $\ket{u}=\widetilde A\ket{\psi}$ and $\ket{v}=\widetilde B\ket{\psi}$. By the Cauchy--Schwarz inequality,
\[
\big|\bra{\psi}\widetilde A\,\widetilde B\ket{\psi}\big|
=
|\langle u|v\rangle|
\le
\|u\|\,\|v\|.
\]
Moreover,
\[
\|u\|^2
=
\bra{\psi}\widetilde A^2\ket{\psi}
=
\bra{\psi}(A-\bar A\mathbb I)^2\ket{\psi}
=
\operatorname{\Std}_\psi(A)^2,
\]
and similarly $\|v\|^2=\operatorname{\Std}_\psi(B)^2$. Combining these identities with \eqref{eq:cov_centered} yields
\[
\big|
\bra{\psi} AB \ket{\psi}
-
\bra{\psi} A \ket{\psi}
\bra{\psi} B \ket{\psi}
\big|
\le
{\operatorname{\Std}_\psi(A)\operatorname{\Std}_\psi(B)},
\]
which proves the claim.
\end{proof}

\begin{lemma}[One-step standard deviation propagation]
\label{lem:variance_propagation}
For any state $\ket{\psi}$ and any $\lambda,\delta\lambda$,
\[
\Std_\psi(\lambda+\delta\lambda)
\le
\Std_\psi(\lambda)
+
|\delta\lambda|
\operatorname{\Std}_\psi(H_{\mathrm f}-H_{\mathrm i}).
\]
\end{lemma}

\begin{proof}
Write
\[
H(\lambda+\delta\lambda)=H(\lambda)+\delta\lambda \mathcal{D},
\qquad
\mathcal{D}=H_{\mathrm f}-H_{\mathrm i}.
\]
Denote expectation values with respect to $\ket{\psi}$ by
$\langle \cdot \rangle = \bra{\psi}(\cdot)\ket{\psi}$.
Then
\[
\Std_\psi(\lambda+\delta\lambda)^2
=
\big\langle (H+\delta\lambda \mathcal{D})^2 \big\rangle
-
\big\langle H+\delta\lambda \mathcal{D} \big\rangle^2 .
\]
Expanding and regrouping terms yields
\begin{align}
\Std_\psi(\lambda+\delta\lambda)^2
&=
\underbrace{\big(\langle H^2\rangle-\langle H\rangle^2\big)}_{=\,V_\psi(\lambda)}
+2\delta\lambda
\big(\langle H\mathcal{D}\rangle-\langle H\rangle\langle \mathcal{D}\rangle\big)
+\delta\lambda^2
\big(\langle \mathcal{D}^2\rangle-\langle \mathcal{D}\rangle^2\big) \notag\\
&=
\Std_\psi(\lambda)^2
+2\delta\lambda\,\mathrm{Cov}_\psi(H,\mathcal{D})
+\delta\lambda^2\,\operatorname{\Std}_\psi(\mathcal{D})^2.
\label{eq:var_expanded}
\end{align}
By Lemma~\ref{lem:covariance_bound},
\[
\big|\mathrm{Cov}_\psi(H,\mathcal{D})\big|
\le
{\operatorname{\Std}_\psi(H)\operatorname{\Std}_\psi(\mathcal{D})}
=
{\Std_\psi(\lambda)\operatorname{\Std}_\psi(\mathcal{D})}.
\]
Inserting this bound into~\eqref{eq:var_expanded} gives
\[
\Std_\psi(\lambda+\delta\lambda)^2
\le
\Std_\psi(\lambda)^2
+2|\delta\lambda|
{\Std_\psi(\lambda)\operatorname{\Std}_\psi(\mathcal{D})}
+\delta\lambda^2\operatorname{\Std}_\psi(\mathcal{D})^2
=
\big(
{\Std_\psi(\lambda)}
+
|\delta\lambda|{\operatorname{\Std}_\psi(\mathcal{D})}
\big)^2.
\]
Taking square roots on both sides yields
\[
{\Std_\psi(\lambda+\delta\lambda)}
\le
{\Std_\psi(\lambda)}
+
|\delta\lambda|{\operatorname{\Std}_\psi(H_{\mathrm f}-H_{\mathrm i})},
\]
which proves the claim.
\end{proof}

\begin{corollary}[Verification condition]
\label{cor:verification_condition}
If
\[
{\Std_\psi(\lambda)}
+
|\delta\lambda|
{\operatorname{\Std}_\psi(H_{\mathrm f}-H_{\mathrm i})}
<
\frac{\deltamin\,}{2}.
\]
In particular, there exists a unique eigen-branch $j_\star$ at $\lambda+\delta\lambda$
such that
\[
\bra{\psi}\Pi_{j_\star}(\lambda+\delta\lambda)\ket{\psi} \ge 8/9.
\]
If $j_\star=0$, this certifies overlap $\ge8/9$ with the actual ground state.
\end{corollary}

\subsubsection*{Verification combined with PŁ tracking}

\begin{theorem}[Certified evolution from PŁ entry and branch verification]
\label{thm:verification_pl_tracking}
Fix $\lambda$ and $\lambda^+=\lambda+\delta\lambda$.
Let $\bth$ be parameters at $\lambda$ with prepared state
$\ket{\psi}=\ket{\psi(\bth)}$.
Define
\[
\delta\lambda_{\rm A} = \frac{\gamma^{2}\deltamin^{2}} {24\,\|H\|_{\mathrm{op}}\, M^{2}\,\|H_\text{f}-H_\text{i}\|_{\mathrm{op}}}, 
\qquad 
\delta\lambda_{\rm V} =\frac{\deltamin/2-\Std_\psi(\lambda)} {\Std_\psi(H_\text{f}-H_\text{i})}.
\]
Assume:
\begin{enumerate}
\item $j_\star=0$;
\item $\Std_\psi(\lambda)\le \deltamin/2$;
\item $\bth$ lies inside the PŁ region at $\lambda$;
\item $|\delta\lambda|\le
\min\{\delta\lambda_{\rm A},\delta\lambda_{\rm V}\}$.
\end{enumerate}
Then:
\begin{enumerate}
\item $\ket{\psi}$ has overlap at least $8/9$ with a unique ground-state branch of
$H(\lambda^+)$;
\item the same parameters $\bth$ lie inside the PŁ region at $\lambda^+$;
\item gradient update steps at $\lambda^+$ contract toward $\bth^\star(\lambda^+)$;
\item if after optimization at $\lambda^+$ the algorithm enforces $\Std_{\psi(\bth_{\mathrm{out}})}(\lambda^+)\le \deltamin/2$, then the output state remains on the same eigen-branch with overlap at least $8/9$.
\end{enumerate}
\end{theorem}

\begin{proof}
Because $|\delta\lambda|\le\delta\lambda_{\rm V}$,
the propagated variance bound
\[
\Std_\psi(\lambda^+)
\le \Std_\psi(\lambda)
+|\delta\lambda|\Std_\psi(H_\text{f}-H_\text{i})
\]
implies $\Std_\psi(\lambda^+)<\deltamin/2$,
so \cref{cor:verification_condition} yields (1).

Because $|\delta\lambda|\le\delta\lambda_{\rm A}$, the drift bound $\|\bth^\star(\lambda^+)-\bth^\star(\lambda)\|\le D|\delta\lambda|$ and the triangle inequality imply that $\bth$ remains within the PŁ radius at $\lambda^+$, giving (2). Statement (3) is the standard PL--Euler contraction. Finally, (4) again follows from Corollary~\ref{cor:verification_condition}.
\end{proof}

% ======================================================
\section{Extension to $\epsilon$-exact representability}
% ======================================================
\label{sec:epsilon_representability}
In the previous analysis, we assumed exact representability of the instantaneous ground state along the adiabatic path. We now relax this assumption and show that the tracking and certification results extend naturally to the case of approximate representability.

\subsubsection*{$\epsilon$-exact representability}
We replace \aref{supp: ass: exact rep} by the following weaker condition.
\begin{assumption}[$\epsilon$-exact representability]
\label{ass:epsilon_representability}
There exists a constant $\epsilon\ge 0$ such that for all
$\lambda\in[0,1]$ there exists parameters $\bar\theta(\lambda)$ satisfying
\begin{equation}
E_\lambda(\bar\theta(\lambda))
\le E_0(\lambda)+\epsilon,
\end{equation}
where $E_0(\lambda)$ denotes the exact ground-state energy.
\end{assumption}

Define the variational optimum
\begin{equation}
\theta^{\mathrm{opt}}(\lambda)
\in \arg\min_\theta E_\lambda(\theta), \qquad
E_\lambda^{\mathrm{opt}} = E_\lambda(\theta^{\mathrm{opt}}(\lambda)).
\end{equation}
By the variational principle,
\begin{equation}
0 \le E_\lambda^{\mathrm{opt}}-E_0(\lambda)
\le \epsilon.
\end{equation}
Thus, in the absence of exact representability, optimization targets the best achievable variational approximation rather than the exact ground state.

\subsubsection*{Ground-state fidelity and representability bias}
Approximate representability affects only statements that attempt to infer ground-state fidelity from optimization alone. Using the gap bound $\deltamin(\lambda)\ge\Delta_c>0$ and the spectral decomposition of $H(\lambda)$, any normalized state $\ket{\psi}$ satisfies
\begin{equation}
1-|\langle \psi_0(\lambda)\mid\psi\rangle|^2 \le \frac{\langle H(\lambda)\rangle_\psi - E_0(\lambda)}{\Delta_c}.
\end{equation}
Applying this bound to the variational optimum yields
\begin{equation}
|\langle \psi_0(\lambda)\mid \psi(\theta^{\mathrm{opt}}(\lambda))\rangle|^2 \ge 1-\frac{\epsilon}{\Delta_c}.
\end{equation}
This term represents an intrinsic expressibility bias that cannot be removed by optimization.

\subsubsection*{PŁ tracking under approximate representability}
Under $\epsilon$-exact representability, the variational minimizer $\theta^{\mathrm{opt}}(\lambda)$ no longer corresponds to the exact ground state, but the local curvature remains strictly positive provided the representability bias is smaller than the spectral gap.

Evaluating the Hessian at $\theta^{\mathrm{opt}}(\lambda)$ and using $E_\lambda^{\mathrm{opt}}-E_0(\lambda)\le \epsilon$ yields
\begin{equation}
\nabla^2 E_\lambda\!\bigl(\theta^{\mathrm{opt}}(\lambda)\bigr) \succeq 2\gamma\bigl(\deltamin - \epsilon\bigr) I .
\end{equation}
Hence, the effective PŁ constant becomes
\begin{equation}
\mu_{\mathrm{eff}} = \gamma\bigl(\deltamin - \epsilon\bigr),
\end{equation}
and the PŁ radius is reduced to
\begin{equation}
r_{\rm PL}^{(\epsilon)} = \frac{\gamma\bigl(\deltamin - \epsilon\bigr)}{L_H}.
\end{equation}
The reduced PL radius also reduces the admissible $\delta\lambda$
\begin{equation}
|\delta\lambda| \le \delta\lambda_{\rm A}^{(\epsilon)} = \frac{\gamma^2\bigl(\deltamin - \epsilon\bigr)^2}
{L_H\sqrt{M}\,\|\partial_\lambda H\|_{\mathrm{op}}}.
\end{equation}
Under the condition
\begin{equation}
\epsilon < \deltamin,
\end{equation}
the PŁ region remains nondegenerate.  All PŁ tracking lemmas and theorems of the supplement then hold as stated with two changes: $\theta^\star(\lambda)$ replaced by $\theta^{\mathrm{opt}}(\lambda)$, and the substitution
\begin{equation}
\deltamin \longrightarrow
\deltamin - \epsilon.
\end{equation}

Thus, approximate representability reduces the effective curvature, shrinks the PŁ region, and tightens the admissible adiabatic step size through the replacement of $\deltamin$ by $\deltamin - \epsilon$.

\subsubsection*{Verification guarantees remain unchanged}
The variance-based certification results of \cref{cor:verification_condition} are purely spectral and do not rely on exact representability. Therefore, if the standard-deviation condition $\Std_\psi(H(\lambda))<\Delta_c/2$ holds, the prepared state obeys
\begin{equation}
|\langle \psi_0(\lambda)\mid\psi(\theta)\rangle|^2 \ge \frac{8}{9},
\end{equation}
independently of $\epsilon$. In particular, approximate representability modifies only the tracking interpretation (optimization toward $\theta^{\mathrm{opt}}$) but does not degrade the certified fidelity bound obtained from runtime verification.

\subsubsection*{Admissible range of the representability error}
\label{subsec:max_eps_rep}
The representability error $\epsilon$ determines whether the variance-based certification condition can be satisfied.
Certification requires
\begin{equation}
\Std_\psi(H(\lambda)) < \frac{\Delta_c}{2},
\end{equation}
equivalently,
\begin{equation}
\Var_\psi(H(\lambda)) < \frac{\Delta_c^2}{4}.
\end{equation}
Suppose the variational ansatz has representability bias
\(
E_\lambda^{\mathrm{opt}} - E_0(\lambda) \le \epsilon.
\)
This bias induces a nonzero minimum achievable variance. Using the spectral decomposition
\[
H(\lambda)=\sum_{j\ge 0} E_j(\lambda)\Pi_j(\lambda),
\qquad
p_j=\langle\psi|\Pi_j(\lambda)|\psi\rangle,
\]
define shifted excitation energies
\[
\delta_j := E_j(\lambda)-E_0(\lambda).
\]
Since variance is invariant under constant shifts,
\[
\Var_\psi(H(\lambda))
=
\sum_{j\ge 0} p_j \delta_j^2
-
\Big(\sum_{j\ge 0} p_j \delta_j\Big)^2.
\]
The gap condition implies
\(
\delta_0=0
\)
and
\(
\delta_j \ge \Delta_c
\)
for all $j\ge1$. Because $\delta_j \in \{0\}\cup[\Delta_c,\infty)$, we have $\delta_j^2 \ge \Delta_c \delta_j$ for all $j$. Hence,
\begin{equation}
\sum_{j\ge 0} p_j \delta_j^2 \ge \Delta_c \sum_{j\ge 0} p_j \delta_j = \Delta_c\bigl(\langle H(\lambda)\rangle_\psi - E_0(\lambda)\bigr).
\end{equation}
Dropping the second (negative) square term yields
\begin{equation}
\Var_\psi(H(\lambda)) \ge \Delta_c\bigl(\langle H(\lambda)\rangle_\psi - E_0(\lambda)\bigr).
\end{equation}
Applying this bound to the variational optimum gives
\begin{equation}
\Var_{\mathrm{opt}}(H(\lambda)) \ge \Delta_c \bigl(E_\lambda^{\mathrm{opt}} - E_0(\lambda)\bigr) \ge \Delta_c \epsilon.
\end{equation}
Therefore,
\begin{equation}
\Std_{\mathrm{opt}}(H(\lambda)) \ge \sqrt{\Delta_c\,\epsilon}.
\end{equation}
Certification requires
\(
\Std_\psi(H(\lambda)) < \Delta_c/2.
\)
Thus, certification can be satisfied whenever
\begin{equation}
\sqrt{\Delta_c\,\epsilon} \le \frac{\Delta_c}{2},
\end{equation}
i.e.
\begin{equation}
\epsilon \le \frac{\Delta_c}{4},
\end{equation}
which is the upper bound on the $\epsilon$-representability error discussed in the main text, since the tracking restriction is less strict.

% ======================================================
\section{Measurement cost and stability under shot noise}\label{sec:measurement_cost}
% ======================================================
In realistic implementations, gradients of the variational energy are not evaluated precisely but are estimated from a finite number of projective measurements on quantum hardware. In this section, we quantify how the required measurement (shot) budget must scale with problem parameters in order to guarantee, with high probability, that (i) all optimization iterates remain inside the local Polyak--\L{}ojasiewicz (P\L{}) region used in the adiabatic tracking analysis, and (ii) the iterates converge toward the \emph{correct} instantaneous variational minimizer along the adiabatic path.

Throughout this section, \(M\) denotes the number of variational parameters and \(\nh\) denotes the number of Pauli measurement terms (or commuting measurement groups) in the Hamiltonian decomposition. We use the explicit PŁ radius established in previous sections,
\begin{equation}
r_{\mathrm{PL}} = \frac{\gamma\deltamin}{L_H}, \qquad L_H = 24\|H\|_{\mathrm{op}} M^{3/2}.
\label{eq:rpl_def}
\end{equation}

% ======================================================
\subsection{Stochastic gradient model induced by finite shot count}
% ======================================================
Fix an adiabatic parameter \(\lambda\) and consider the variational energy
\[
E_\lambda(\bth) = \langle \psi(\bth) | H(\lambda) | \psi(\bth) \rangle, \qquad H(\lambda)=\sum_{\ell=1}^{\nh} h_\ell(\lambda) P_\ell ,
\]
where \(P_\ell\) are Pauli operators defined in the setup \sref{sec: setup}. Using the parameter-shift rule, gradient descent updates take the stochastic form
\begin{equation}
\bth^{(k+1)} = \bth^{(k)} - \eta \bigl( \nabla E_\lambda(\bth^{(k)}) + \xi_k \bigr),
\label{eq:sgd_update_shots}
\end{equation}
where \(\xi_k\) denotes the gradient estimation error induced by finite measurement shots. We assume
\begin{equation}
\mathbb{E}[\xi_k \mid \bth^{(k)}] = 0, \qquad \mathbb{E}\!\left[ \|\xi_k\|_2^2 \mid \bth^{(k)} \right] \le \sigma^2(S),
\label{eq:noise_model}
\end{equation}
where \(S\) is the number of shots per Hamiltonian term. For Pauli measurements with independent shot noise, we can derive an explicit bound on the variance of a single energy estimate. Fix \(\lambda\) and \(\bth\) and  write
\[
E_\lambda(\bth)=\sum_{\ell=1}^K h_\ell(\lambda)\,\langle P_\ell\rangle_{\bth,\lambda},
\]
where \(\langle P_\ell\rangle_{\bth,\lambda}=\langle\psi(\bth)|P_\ell|\psi(\bth)\rangle\in[-1,1]\).
Assume we estimate each Pauli expectation value \(\langle P_\ell\rangle_{\bth,\lambda}\) by performing \(S\) shots of the measurement of \(P_\ell\),
yielding outcomes \(X_{\ell,1},\dots,X_{\ell,S}\in\{+1,-1\}\) with
\[
\mathbb{E}[X_{\ell,s}]=\langle P_\ell\rangle_{\bth,\lambda}, \qquad \mathrm{Var}(X_{\ell,s}) = 1-\langle P_\ell\rangle_{\bth,\lambda}^2 \le 1 .
\]
Define the sample mean estimator
\[
\widehat{\langle P_\ell\rangle} =\frac{1}{S}\sum_{s=1}^S X_{\ell,s}, \qquad \widehat{E_\lambda(\bth)}=\sum_{\ell=1}^K h_\ell(\lambda)\,\widehat{\langle P_\ell\rangle}.
\]
Then \(\widehat{E_\lambda(\bth)}\) is unbiased:
\[
\mathbb{E}\!\left[\widehat{E_\lambda(\bth)}\right] =\sum_{\ell=1}^K h_\ell(\lambda)\,\mathbb{E}\!\left[\widehat{\langle P_\ell\rangle}\right] =\sum_{\ell=1}^K h_\ell(\lambda)\,\langle P_\ell\rangle_{\bth,\lambda} =E_\lambda(\bth).
\]
To bound the variance, first note that, by independence of shots for a fixed \(\ell\),
\[
\mathrm{Var}\!\left(\widehat{\langle P_\ell\rangle}\right) = \mathrm{Var}\!\left(\frac{1}{S}\sum_{s=1}^S X_{\ell,s}\right) = \frac{1}{S^2}\sum_{s=1}^S \mathrm{Var}(X_{\ell,s}) = \frac{1}{S}\mathrm{Var}(X_{\ell,1}) = \frac{1-\langle P_\ell\rangle_{\bth,\lambda}^2}{S} \le \frac{1}{S}.
\]
Next, assume that the estimators \(\widehat{\langle P_\ell\rangle}\) are obtained from independent measurement data across different \(\ell\) (e.g.\ by allocating disjoint shot batches per term or per commuting group). Then the random variables \(\widehat{\langle P_\ell\rangle}\) are independent, and therefore
\begin{align}
\mathrm{Var}\!\left[\widehat{E_\lambda(\bth)}\right]
&= \mathrm{Var}\!\left[\sum_{\ell=1}^\nh h_\ell(\lambda)\,\widehat{\langle P_\ell\rangle}\right] = \sum_{\ell=1}^\nh h_\ell(\lambda)^2\,\mathrm{Var}\!\left(\widehat{\langle P_\ell\rangle}\right) \label{eq:var_sum_indep} \\
&\le \sum_{\ell=1}^\nh h_\ell(\lambda)^2 \cdot \frac{1}{S} = \frac{1}{S}\sum_{\ell=1}^\nh h_\ell(\lambda)^2 = \frac{\|h(\lambda)\|_2^2}{S},
\end{align}
where we defined
\[
\|h(\lambda)\|_2^2 = \sum_{\ell=1}^\nh h_\ell(\lambda)^2.
\]
If measurements are grouped into commuting sets, the same derivation holds with \(\ell\) indexing the groups and \(h_\ell(\lambda)P_\ell\) replaced by the corresponding grouped observable. 

A full parameter-shift gradient requires \(2M\) energy evaluations. Summing the variances of the gradient components yields
\begin{equation}
\sigma^2(S) \le \frac{2M \, \sup_{\lambda \in [0,1]} \|h(\lambda)\|_2^2}{S}.
\label{eq:sigma_scaling_ps}
\end{equation}

% ======================================================
\subsection{High-probability invariance of the PŁ region (never leave PŁ region)}
% ======================================================
Fix \(\lambda\) and write \(\bth^\star=\bth^\star_\lambda\). Throughout this section, we work inside the PŁ region (see \lref{lem: PŁ inequality})
\[
\mathcal D_\lambda = \{\bth:\ \|\bth-\bth^\star\|_2\le r_{\mathrm{PL}}\}, \qquad r_{\mathrm{PL}}=\frac{\gamma\deltamin}{L_H}, \qquad \mu=\gamma\deltamin ,
\]
Consider the stochastic update 
\begin{equation}
\bth^{(k+1)}=\bth^{(k)}-\eta\bigl(\nabla E_\lambda(\bth^{(k)})+\xi_k\bigr), \qquad \eta\le \frac{1}{L},
\label{eq:sgd_update_recall}
\end{equation}
where $L$ is the smoothness constant defined in \lref{lem: smoothness}.

By the triangle inequality applied to~\eqref{eq:sgd_update_recall},
\begin{align}
\|\bth^{(k+1)}-\bth^\star\|_2
&= \bigl\|\bth^{(k)}-\bth^\star-\eta\nabla E_\lambda(\bth^{(k)})-\eta\xi_k\bigr\|_2 \notag\\
&\le \underbrace{\|\bth^{(k)}-\bth^\star-\eta\nabla E_\lambda(\bth^{(k)})\|_2}_{\text{noiseless GD step}} +\eta\|\xi_k\|_2.
\label{eq:inv_triangle}
\end{align}
Inside \(\mathcal D_\lambda\), PL\(+\)smoothness implies that gradient descent with \(\eta\le 1/L\) is contractive in distance to \(\bth^\star\) (see \lref{lem: warm-start}):
\begin{equation}
\|\bth^{(k)}-\bth^\star-\eta\nabla E_\lambda(\bth^{(k)})\|_2 \le \sqrt{1-\eta\mu}\|\bth^{(k)}-\bth^\star\|_2.
\label{eq:inv_contraction}
\end{equation}
Combining~\eqref{eq:inv_triangle}--\eqref{eq:inv_contraction} and using \(\|\bth^{(k)}-\bth^\star\|_2\le r_{\mathrm{PL}}\) gives
\[
\|\bth^{(k+1)}-\bth^\star\|_2 \le \sqrt{1-\eta\mu}\, r_{\mathrm{PL}}+\eta\|\xi_k\|_2.
\]
Thus \(\|\bth^{(k+1)}-\bth^\star\|_2\le r_{\mathrm{PL}}\) is guaranteed whenever \(\sqrt{1-\eta\mu}\,r_{\mathrm{PL}}+\eta\|\xi_k\|_2< r_{\mathrm{PL}}\). For small $\eta\,\mu$ we find 
\begin{equation}\label{eq:noise_abs_opt}
\|\xi_k\|_2<\frac12 \mu\, r_{\mathrm{PL}}.
\end{equation}
This condition is \emph{tight};  if \(\|\xi_k\|_2>\frac12\mu r_{\mathrm{PL}}\), then for a point on the boundary
\(\|\bth^{(k)}-\bth^\star\|_2=r_{\mathrm{PL}}\) the upper bound \eref{eq:inv_triangle} exceeds \(r_{\mathrm{PL}}\), so one-step invariance cannot be ensured uniformly over all boundary points.

\subsubsection*{High-probability enforcement via Gaussian norm concentration.}
Assume that, conditionally on \(\bth^{(k)}\), the gradient noise is Gaussian with mean zero and isotropic covariance
chosen so that it matches the variance proxy in \eqref{eq:noise_model}:
\begin{equation}
\xi_k \mid \bth^{(k)} \sim \mathcal N\!\left(0,\;\frac{\sigma^2(S)}{M} I_M\right),
\qquad\text{so that}\qquad
\mathbb E\!\left[\|\xi_k\|_2^2\mid \bth^{(k)}\right]=\sigma^2(S).
\label{eq:gaussian_noise_assumption}
\end{equation}
Equivalently, we may write \(\xi_k = \frac{\sigma(S)}{\sqrt M}\,g_k\) with \(g_k\sim \mathcal N(0,I_M)\).
\medskip
Since the map \(g\mapsto \|g\|_2\) is \(1\)-Lipschitz and \(g_k\) is standard Gaussian, we have for all \(x\ge 0\)
\begin{equation}
\mathbb P\!\left(\|g_k\|_2 \ge \mathbb E\|g_k\|_2 + \sqrt{2x}\right)\le e^{-x}.
\label{eq:gaussian_lipschitz}
\end{equation}
Moreover, \(\mathbb E\|g_k\|_2 \le \sqrt{M}\). Therefore, for all \(x\ge 0\),
\begin{equation}
\mathbb P\!\left(\|g_k\|_2 \ge \sqrt{M} + \sqrt{2x}\right)\le e^{-x}.
\label{eq:gaussian_norm_tail}
\end{equation}
Rescaling back to \(\xi_k=\frac{\sigma(S)}{\sqrt M}g_k\) yields
\begin{equation}
\mathbb P\!\left(
\|\xi_k\|_2 \ge \sigma(S)\Bigl(1+\sqrt{\tfrac{2x}{M}}\Bigr)
\;\middle|\; \bth^{(k)}
\right)
\le e^{-x}.
\label{eq:xi_norm_tail}
\end{equation}
Set \(x=\log(K/\delta)\).
Then \eqref{eq:xi_norm_tail} gives
\[
\mathbb P\!\left(
\|\xi_k\|_2 \ge \sigma(S)\Bigl(1+\sqrt{\tfrac{2\log(K/\delta)}{M}}\Bigr)
\;\middle|\; \bth^{(k)}
\right)
\le \frac{\delta}{K}.
\]
Applying a union bound over \(k=0,\dots,K-1\), we obtain that with probability at least \(1-\delta\),
\begin{equation}
\|\xi_k\|_2 \le \sigma(S)\Bigl(1+\sqrt{\tfrac{2\log(K/\delta)}{M}}\Bigr)
\qquad\text{for all }k=0,\dots,K-1.
\label{eq:xi_uniform_bound}
\end{equation}
Combining \eqref{eq:xi_uniform_bound} with the deterministic invariance condition
\(\|\xi_k\|_2 < \frac12 \,\mu r_{\mathrm{PL}}\) from \eref{eq:noise_abs_opt}, it suffices that
\begin{equation}
\sigma(S)\Bigl(1+\sqrt{\tfrac{2\log(K/\delta)}{M}}\Bigr)
\le \frac12\,\mu r_{\mathrm{PL}}.
\label{eq:sigma_invariance_correct}
\end{equation}
Equivalently,
\begin{equation}
\sigma(S)
\le
\frac12\,\frac{\mu r_{\mathrm{PL}}}{
1+\sqrt{\tfrac{2\log(K/\delta)}{M}}
}.
\label{eq:sigma_invariance_correct_solved}
\end{equation}
Using the parameter-shift variance proxy \(\sigma^2(S)\le \dfrac{2M\sup_\lambda\|h(\lambda)\|_2^2}{S}\), a sufficient shot budget is therefore
\begin{equation}
S \ge \frac{8M\sup_\lambda\|h(\lambda)\|_2^2}{\mu^2 r_{\mathrm{PL}}^2} \left( 1+\sqrt{\tfrac{2\log(K/\delta)}{M}} \right)^2.
\label{eq:shots_invariance_correct}
\end{equation}
Substituting \(\mu=\gamma\deltamin\) and \(r_{\mathrm{PL}}=\gamma\deltamin/L_H\) yields the gap scaling
\begin{equation}
\boxed{S\ge \frac{8M\sup_\lambda\|h(\lambda)\|_2^2\,L_H^2}{\gamma^4\deltamin^4} \left( 1+\sqrt{\tfrac{2\log(K/\delta)}{M}} \right)^2}\,.
\label{eq:shots_invariance_gap_scaling_correct}
\end{equation}
In particular, the leading dependence on the spectral gap is \(S\propto \deltamin^{-4}\).

% ======================================================
\subsection{Total measurement cost}
% ======================================================
Each parameter-shift gradient evaluation requires \(2M\) energy measurements.
Each energy measurement consists of \(\nh\) Pauli terms estimated with \(S\) shots.
Therefore, the measurement cost per gradient step is
\[
\mathcal{C}_{\mathrm{iter}} = 2\,M\,\nh \,S .
\]
Over \(K\) gradient updates, the total measurement cost (for fixed $\lambda$) is
\begin{equation}
\mathcal{C}_{\mathrm{total}} = 2\,K\,M\,\nh\, S ,
\end{equation}
with \(S\) chosen according to~\eqref{eq:shots_invariance_gap_scaling_correct}.

\subsubsection*{Summary}
When the PŁ radius is fixed to its explicit value \(r_{\mathrm{PL}}=\gamma\deltamin/L_H\), finite-shot noise does not invalidate adiabatic PL-based tracking, provided the shot budget scales polynomially in \(M\), \(K\), and the inverse gap. With parameter-shift gradients, both high-probability invariance of the PŁ region and convergence to the correct instantaneous minimizer are guaranteed under an explicit and controlled measurement budget.

\bibliography{references}

\end{document}
